# Supplementary material for: Decentralized Optimization On Time-Varying Directed Graphs Under Communication Constraints
Source: arXiv:2005.13189 source file (2021-08-30)
Supplement: Supplementary file 1 [file appendix.tex]

\section*{Appendices}
The appendix is organized as follows: Appendix \ref{app:A} and Appendix \ref{app:B} present the analysis of the consensus and optimization problems, respectively; Section Appendix \ref{app:C} discusses the effect of compression rate on Erdős–Rényi random graphs; Section Appendix \ref{app:D} provides further simulation results and provides details about the benchmark algorithms.

\section{Consensus Problem}\label{app:A}
% \subsection{A.1. Proof of Lemma $1$}
% See \cite{cai2012average}.
\subsection{Elaborating on Assumption \ref{assumption0}}\label{app:A1}

Analysis of the algorithms presented in the paper is predicated on the property of the product of consecutive mixing matrices of general time-varying graphs stated in Assumption \ref{assumption0}. Here we establish conditions under which this property holds for a specific graph structure, i.e., identify $\epsilon_0$ in Assumption \ref{assumption0} for the graphs that are jointly connected over $\mathcal{B}$ consecutive time steps. Note that when $\mathcal{B}=1$, such graphs reduce to the special case of graphs that are strongly connected at each time step. For convenience, we formally state the $\mathcal{B} > 1$ and $\mathcal{B}=1$ settings as Assumption \ref{assumption1} and \ref{assumption1'}, respectively.

%{\color{red}{ISN'T ASSUMPTION 1 COROLLARY OF Lemma \ref{lemma0} (I.E., FOLLOW FROM Lemma \ref{lemma0})? IF IT IS, THEN IT SHOULD NOT BE CALLED ``ASSUMPTION" (ASSUMPTIONS ARE NOT PROVED, RIGHT?).}}
%{\color{blue}{I leave this as an assumption because it is actually a weaker assumption than assumption 2. Assumption 2 is not a necessary condition for which assumption 1 holds. I understand that assumption 1 is not straightforward because it is not describing the graph structure directly and I am still thinking about some intuitions for it. }}

%Note that Assumption \ref{assumption0} is satisfied for a range of values of the perturbation parameter $\epsilon$ given $\mathcal{B}$-jointly-connected network for $\mathcal{B} \geq 1$ (see the following two assumptions). 

%Note that the above network connectivity assumption may not be necessary in cases where a properly specified $\epsilon$ can guarantee a non-zero spectral gap even if the network is not jointly-connected. 
%{\color{red}{THIS STATEMENT SHOULD BE EXPANDED/CLARIFIED AND MADE MORE PRECISE.}}
%{\color{blue}{Does this refer to some numerical examples?}}

\begin{assumption}\label{assumption1}
The graphs $\G_m(t)=(|n|, \E_m(t))$,
modeling network connectivity for the $m\ts{th}$ entry of the sparsified parameter vectors, are $\mathcal{B}$-jointly-connected. 
\end{assumption}

Assumption~\ref{assumption1}
implies that starting from any time step $t = k\mathcal{B}$, $k \in \mathcal{N}$, the union graph over $\mathcal{B}$ consecutive time steps is a strongly connected graph. This is a weaker requirement then the standard assumption (Assumption~\ref{assumption1'} given below) often encountered in literature on convergence analysis of algorithms for distributed optimization and consensus problems.

\begin{assumption}\label{assumption1'}
The graphs $\G_m(t)=(|n|, \E_m(t))$,
modeling network connectivity for the $m\ts{th}$ entry of the sparsified parameter vectors, are strongly connected at any time $t$. 
\end{assumption}

 Next, we state a lemma adopted from \cite{cai2012average} which helps establish that under Assumptions \ref{assumption2} and \ref{assumption1'}, the so-called spectral gap of the product of mixing matrices taken over a number of consecutive time steps is non-zero. 
 
\begin{lemma}\label{lemma1}
\cite{cai2012average} Suppose Assumptions \ref{assumption2} and \ref{assumption1'} hold. Let $M_m^t$ be the mixing matrix in \eqref{matrixdef} such that $\epsilon \in (0,\gamma_m)$, where $\gamma_m = \frac{1}{(20+8n)^n}(1-|\lambda_3(\Bar{M}_m^t)|)^n$. Then, the mixing matrix $M_m^t$ has a simple eigenvalue $1$ and all its other eigenvalues have magnitude smaller than $1$.
\end{lemma}
 %%%%%%%%%%%%%%%%%%%%%%%%%%%%%%%%%%%%%%%%%%%%%
 %%%%%%%%%%%%%%%%%%%%%%%%%%%%%%%%%%%%%%%%%%%%
Note that Lemma \ref{lemma1} implies that 
\begin{equation}
    \label{Mlim}
    \mathrm{lim}_{k \to \infty}(M_m^t)^k=\left[\begin{matrix}
    \frac{\mathbf{1}_n \mathbf{1}^T_n}{n} & \frac{\mathbf{1}_n \mathbf{1}^T_n}{n} \\
    \mathbf{0} & \mathbf{0} \\
  \end{matrix}
\right],
\end{equation}
where the rate of convergence is geometric and determined by the nonzero spectral gap of the perturbed mixing matrix $M_m^t$, i.e., $1-|\lambda_2(M_m^t)|$. This implies that the local estimate, $x^t_{im}$, approaches the average consensus value $\Bar{z}^t_{m}=\frac{1}{n}\sum_{i=1}^n x^t_{im}+\frac{1}{n}\sum_{i=1}^n y^t_{im}$ while the auxiliary variable $y^t_{im}$ vanishes to 0.
 
We now utilize the insight of (\ref{Mlim}) to establish a
result that will facilitate convergence analysis of the setting described by Assumption~\ref{assumption1}. In particular, we consider the setting where in any time window of size $\mathcal{B}$ starting from time $t = k\mathcal{B}$ for some integer $k$, the union of the associated directed graphs is strongly connected.
 The following lemma will help establish that if a small perturbation, 
%  \[
%  \epsilon F = \begin{bmatrix}
%  0 & \epsilon I \\
%  0 & -\epsilon I
%  \end{bmatrix},
%  \]
$\epsilon F$
 is added to the product of mixing matrices  $\bar{M}_m((k+1)\mathcal{B}-1:k\mathcal{B} ) $ 
 %(see \eqref{eq:update_consensus})
 , then
 the product $M_m((k+1)\mathcal{B}-1:k\mathcal{B} )$ has only a simple eigenvalue $1$ while all its other eigenvalues have moduli smaller than one.

\begin{lemma}\label{lemma2}
Suppose that Assumptions \ref{assumption2} and \ref{assumption1} hold. 
If the parameter $\epsilon \in (0, \bar{\epsilon})$ and $\bar{\epsilon} = \min_m \gamma_m$, where $\gamma_{m} = \min_k \frac{1}{(20+8n)^n}(1-|\lambda_3(\bar{M}_m((k+1)\mathcal{B}-1:k\mathcal{B}))|)^n$, then for each $m$ the mixing matrix product $M_m((k+1)\mathcal{B}-1:k\mathcal{B} ) $ has simple eigenvalue $1$ for all integer $k \geq 0$ and $\epsilon \in (0,  \bar{\epsilon})$.
\end{lemma}
 
\begin{proof}
Consider a fixed realization of $\mathcal{B}$-strongly-connected graph sequences,\newline $\left\{\G(0), \cdots, \G(\mathcal{B}-1) \right\}.$
For $s \in 0, \cdots, \mathcal{B}-1$, $\bar{M}^s$ is block (lower) triangular and the spectrum is determined by the spectrum of the $(1, 1)$-block and the $(2, 2)$-block. Furthermore, for such $s$, $A^s$ (row-stochastic) and $B^s$ (column-stochastic) matrices have non-negative entries. Owing to the fact that the union graph over $\mathcal{B}$ iterations is strongly connected, $\Pi_{s=0}^{\mathcal{B}-1 }A^s = A^{\mathcal{B}-1}\cdots A^0 $ and $\Pi_{s=0}^{\mathcal{B}-1 }B^s = B^{\mathcal{B}-1}\cdots B^0 $ are both irreducible. Thus, $\Pi_{s=0}^{\mathcal{B}-1 }A^s $ and $\Pi_{s=0}^{\mathcal{B}-1 }B^s$ both have simple eigenvalue $1$. Recall that $\Pi_{s=0}^{\mathcal{B}-1 }\bar{M}^s$ has column sum equal to $1$, and thus we can verify that $\mathrm{rank}(\Pi_{s=0}^{\mathcal{B}-1 }\bar{M}^s - I)=2n-2$; therefore, the eigenvalue $1$ is semi-simple.
 \\~\\
Next, we characterize the change of the semi-simple eigenvalue $\lambda_1 = \lambda_2 = 1$ of $\Pi_{s=0}^{\mathcal{B}-1 }\bar{M}^s$ when a small perturbation $\epsilon F$ is added. Consider the eigenvalues of the perturbed matrix product,  $\lambda_1(\epsilon)$, $\lambda_2(\epsilon) $, which corresponds to $ \lambda_1$, $\lambda_2$, respectively. 
For all $s \in 0, \cdots, \mathcal{B}-1$, $ \bar{M}^s$ has two common right eigenvectors and left eigenvectors for eigenvalue $1$; they are the right eigenvectors and left eigenvectors of the matrix product. The right eigenvectors $y_1$, $y_2$ and left eigenvectors $z_1$, $z_1$ of the semi-simple eigenvalue $1$ are
 \begin{equation}
     Y := \begin{matrix}[y_1 & y_2]\end{matrix} = \begin{bmatrix} 0 & 1 \\ v_2 & -nv_2 \end{bmatrix}, \quad\hspace{-2mm} Z := \begin{bmatrix}z_1' \\ z_2'\end{bmatrix} = \begin{bmatrix} 1' & 1' \\ v_1' & 0 \end{bmatrix}.
 \end{equation}
 By following exactly the same steps and using Proposition $1$ in \cite{cai2012average}, we can show that for small $\epsilon >0$, the perturbed matrix product has a simple eigenvalue $1$. Further, it can be guaranteed that for $\epsilon < \frac{1}{(20+8n)^n}(1-|\lambda_3(\bar{M}(\mathcal{B}-1:0)|)^n$, the perturbed matrix product $M(\mathcal{B}-1:0 ) $ has simple eigenvalue $1$. 
 \\~\\
From Assumption \ref{assumption2}, there is only a finite number of possible mixing matrices $\left\{\bar{M}^t_m \right\}$; if we let $\gamma_{m} = \min_k \frac{1}{(20+8n)^n}(1-|\lambda_3(\bar{M}_m((k+1)\mathcal{B}-1:k\mathcal{B}))|)^n$, starting from any time step $t = k\mathcal{B}$, the perturbed mixing matrix product $M_m(t+\mathcal{B}-1:t ) $ has simple eigenvalue $1$ for all $\epsilon < \bar{\epsilon} = \min_m \gamma_m$.
 \end{proof}
	
\subsection{Proof of Lemma $1$}

% For convenience, we repeat the statement of Lemma \ref{lemma0}.

% \newtheorem*{lemma1}{Lemma $1$}
% \begin{lemma1}
% Suppose that Assumptions \ref{assumption0} and \ref{assumption2} hold. 
% There exist $\epsilon_0 >0$ such that if $\epsilon \in (0, \epsilon_0)$
% then for all $m = 1, \cdots, d$ the following statements hold.
 
% \begin{enumerate}[(a)]
% \item The spectral norm of 
% $M_m((k+1)\mathcal{B}-1:k\mathcal{B})$ satisfies
% \begin{equation*}
% \begin{aligned}
% \rho(M_m((k+1)\mathcal{B}-1:k\mathcal{B})) - \frac{1}{n}[\mathbf{1}^T \ \mathbf{0}^T]^T[\mathbf{1}^T \  \mathbf{1}^T]) 
%      = \sigma <1
%      \end{aligned}
% %     \rho(\bar{M}((s+1)\mathcal{B}-1:s\mathcal{B}))+\epsilon F - \frac{1}{n}[\mathbf{1}^T \ \mathbf{0}^T]^T[\mathbf{1}^T \  \mathbf{1}^T]) = \sigma <1
%      \end{equation*}
%      $\forall k \in \mathcal{N}$.
% \item 
% There exists $\Gamma = \sqrt{2nd}>0$ such that
% \begin{equation*}
%     \|
%     M_m(n\mathcal{B}-1:0)-\frac{1}{n}[\mathbf{1}^T \ \mathbf{0}^T]^T[\mathbf{1}^T \  \mathbf{1}^T]\|_{\infty} \leq \Gamma \sigma^{n}.
%     \end{equation*}
%  \end{enumerate}
% \end{lemma1}

%\begin{proof}
We start this proof by introducing two intermediate lemmas: Lemma \ref{lemma11} and Lemma \ref{lemma12}. 
	
%	Next, we continue proving this lemma using the following intermediate lemma:
\begin{adjustwidth}{0.25cm}{0cm}\qquad
\begin{lemma}\label{lemma11}
% \begin{lemma}
Assume that $M_m((s+1)\mathcal{B}-1:s\mathcal{B})$ has non-zero spectral gap for each $m$.
%the selection of communicating nodes still constructs a jointly-connected graph and $M_m((s+1)\mathcal{B}-1:s\mathcal{B})$ is product of mixing matrices with respect to the entry position $m$, defined as in the main paper. 
Then the following statements hold.
\begin{enumerate}[(a)]
\item The sequence of matrix products $M_m((s+1)\mathcal{B}-1:s\mathcal{B})$ converges to the limit matrix
\begin{equation}
\mathrm{lim}_{t \to \infty} (M_m((s+1)\mathcal{B}-1:s\mathcal{B}))^t=
\left[\begin{matrix}
\frac{\mathbf{1}_n \mathbf{1}^T_n}{n} & \frac{\mathbf{1}_n \mathbf{1}^T_n}{n} \\
\mathbf{0} & \mathbf{0} \\
\end{matrix}
\right].
\end{equation}
\item Let $1=|\lambda_1(M_m((s+1)\mathcal{B}-1:s\mathcal{B}))|>|\lambda_2(M_m((s+1)\mathcal{B}-1:s\mathcal{B}))|\geq \cdots \geq |\lambda_{2n}(M_m((s+1)\mathcal{B}-1:s\mathcal{B}))|$ be the eigenvalues of $M_m((s+1)\mathcal{B}-1:s\mathcal{B})$, and let $\sigma_m=|\lambda_2(M_m((s+1)\mathcal{B}-1:s\mathcal{B}))|$; then there exists $\Gamma_m'>0$ such that
\begin{equation}
\begin{aligned}
\|(M_m((s+1)\mathcal{B}-1:s\mathcal{B}))^t-\mathcal{I}\|_{\infty} 
\leq \Gamma_m' \sigma_m^{t},
\end{aligned}
\end{equation}
where $\mathcal{I}:=\frac{1}{n}[\mathbf{1}^T \ \mathbf{0}^T]^T[\mathbf{1}^T \  \mathbf{1}^T]$.
\end{enumerate}
\end{lemma}
	% \end{lemma}
	
\begin{proof}
For each $m$, $M_m((s+1)\mathcal{B}-1:s\mathcal{B})$ has column sum equal to $1$. According to Assumption \ref{assumption0}, definition of the mixing matrix (\ref{matrixdefbar}), and the construction of the product (\ref{mproduct}),
$M_m((s+1)\mathcal{B}-1:s\mathcal{B})$ has a simple eigenvalue $1$ with the corresponding left eigenvector $[\mathbf{1}^T \ \mathbf{1}^T]$ and right eigenvector $[\mathbf{1}^T \ \mathbf{0}^T]^T$.
Following Jordan matrix decomposition for the simple eigenvalue, there exist some $P, Q \in \mathcal{R}^{(2n-1)\times (2n-1)}$ such that
	\begin{equation}
	\begin{aligned}
	(M_m((s+1)\mathcal{B}-1:s\mathcal{B}))^t & =\mathcal{I}^t+P J_m^t Q
	=\mathcal{I}+P J_m^t Q. 
	\end{aligned}
%	(M_m((s+1)\mathcal{B}-1:s\mathcal{B}))^t=(\frac{1}{n}[\mathbf{1}^T \ \mathbf{0}^T]^T[\mathbf{1}^T \ \mathbf{1}^T])^t+P J_m^t Q =\frac{1}{n}[\mathbf{1}^T \ \mathbf{0}^T]^T[\mathbf{1}^T \ \mathbf{1}^T]+P J_m^t Q 
\end{equation}
Let $\gamma_m$ be the second largest eigenvalue magnitude of $M_m((s+1)\mathcal{B}-1:s\mathcal{B})$; then, $\gamma_m$ is also the spectral norm of $J_m$. The proof of part (a) follows by noting that 
$
\mathrm{lim}_{t \to \infty}J_m^t = \mathbf{0}.
$
Since $\|P \|$, $\| Q \|$ and $\|J_m \|$ are finite, there exists some $\Gamma_m' >0$ such that
\begin{equation}
\begin{aligned}
& \quad \|(M_m((s+1)\mathcal{B}-1:s\mathcal{B}))^t-\mathcal{I} \|_{\infty} 
\leq \|P J_m^t Q \|_{\infty} 
%\leq \|P \|_{\infty} \|Q \|_{\infty} \|J_m^t \|_{\infty} 
\leq \Gamma_m' \sigma_m^t
\end{aligned}
%	\|(M_m((s+1)\mathcal{B}-1:s\mathcal{B}))^t-\frac{1}{n}[\mathbf{1}^T \ \mathbf{0}^T]^T[\mathbf{1}^T \ \mathbf{1}^T] \|_{\infty} \leq \|P J_m^t Q \|_{\infty} \leq \|P \|_{\infty} \|Q \|_{\infty} \|J_m^t \|_{\infty} \leq \Gamma_m' \sigma_m^t
\end{equation}
which completes the proof of part (b).
\end{proof}

% newtheorem*{lemma1''}{Lemma $1''$}
%	Fix $\epsilon \in (0, \gamma)$ where $\gamma$ is defined as in Lemma \ref{lemma3} 
\begin{lemma}\label{lemma12}
Suppose that for each $m$, $M_m((s+1)\mathcal{B}-1:s\mathcal{B})$ has non-zero spectral gap. Let $\sigma = \max_m \sigma_m$, where $\sigma_m$ is as defined in Lemma \ref{lemma11}.
	%$\gamma = \frac{1}{(20+8n)^n}(1-|\lambda_3|)^n$.
	%Denote the set of all possible mixing matrices as $\left\{M_1(\epsilon), \cdots, M_N(\epsilon) \right\}$, at iteration $t$, the constructed mixing matrix $M^t \in \left\{M_1(\epsilon), \cdots, M_N(\epsilon) \right\}$. Denote $\sigma_2=\mathrm{max}\left\{|\lambda_2(M_1(\epsilon) )|, \cdots, |\lambda_2(M_N(\epsilon) )| \right\}$, 
Then, for each $m$ it holds that
\begin{equation}
\rho (M_m(T\mathcal{B}-1:0)-\frac{1}{n}[\mathbf{1}^T \ \mathbf{0}^T]^T[\mathbf{1}^T \  \mathbf{1}^T]) \leq  \sigma^{T}.
\end{equation}
%where $\rho(A)$ represents the spectral norm of matrix $A$.
\end{lemma}
\begin{proof}
We prove this lemma by induction. \\~\\
\textbf{Base step.} $T=1$. According to the selection rule of $M_m(\mathcal{B}-1:0)$ and definition of $\sigma$, the statement holds. \\~\\
\textbf{Inductive step.} Suppose for all $T_1 < T$ the statement holds. Let $T_1=T$. Since for each time step $t = k\mathcal{B}$,  $M_m(t\mathcal{B}-1:(t-1)\mathcal{B})$ has column sum equal to $1$ and has a simple eigenvalue $1$ with the corresponding left eigenvector $[\mathbf{1}^T \ \mathbf{1}^T]$ and right eigenvector $[\mathbf{1}^T \ \mathbf{0}^T]^T$, then 
\begin{align*}
 \quad M_m(T\mathcal{B}-1:0)-\mathcal{I} & =M_m(T\mathcal{B}-1:0) -\mathcal{I}M_m(\mathcal{B}-1:0) \\
 & = (M_m(T\mathcal{B}-1:\mathcal{B})-\mathcal{I} )M_m(\mathcal{B}-1:0). 
	\end{align*}
Taking the spectral norm over both hand sides after recursion and applying Gelfand corollaries, we complete the proof. \end{proof}
\end{adjustwidth}

%\textbf{Proof of Lemma $1$:} 
We now continue with the proof of Lemma \ref{lemma0}.
Lemma \ref{lemma12} implies the result in part (a) of Lemma \ref{lemma0}. Due to the equivalence of matrix norms, we can obtain the desired results in Lemma \ref{lemma0} (b). In particular, for matrix $A\in \mathcal{R}^{m \times n}$ it holds that \begin{equation*}
    \frac{1}{\sqrt{n}} \|A \|_{\infty}\leq \|A \|_2 \leq \sqrt{m} \|A \|_{\infty}.
\end{equation*}
Since Lemma \ref{lemma12} shows that
$
\|M_m(T\mathcal{B}-1:0)-\mathcal{I} \|_2 \leq \sigma^T,
$
then there exists $\Gamma = \sqrt{2nd} >0$ such that
\begin{equation*}
    \|M_m(T\mathcal{B}-1:0)-\frac{1}{n}[\mathbf{1}^T \ \mathbf{0}^T]^T[\mathbf{1}^T \  \mathbf{1}^T] \|_{\infty} \leq \Gamma \sigma^T,
\end{equation*}
which completes the proof. 
%\end{proof}
	
\subsection{Proof of Theorem \ref{theorem1}}
	
% \newtheorem*{Theorem1}{Theorem \ref{theorem1}}
% \begin{Theorem1}
% Suppose Assumptions \ref{assumption0} and \ref{assumption2} hold, and instate the notations and hypotheses above. Then, there exist $\sigma \in (0, 1)$ and $\Gamma = \sqrt{2nd}$ such that the following statements hold.
% \begin{enumerate}[(a)]
%     \item For $1 \leq i \leq n$ and $t = k\mathcal{B} - 1 + t'$, where $t' = 0, \cdots, \mathcal{B}-1$,
%     \begin{equation*}
%     \|\mathbf{z}_i^t-\mathbf{\Bar{z}}\| \leq \Gamma \sigma^{k} \sum_{j=1}^{2n}\sum_{m=1}^d |z^0_{jm}|,
%     \end{equation*}
%     and
%     \begin{equation*}
%     \|\mathbf{z}_i^t-\mathbf{\Bar{z}}\| \leq \Gamma (\sigma^{1/\mathcal{B}})^{t-(t'-1) } \sum_{j=1}^{2n}\sum_{m=1}^d |z^0_{jm}|,
%     \end{equation*}
%     where $\mathbf{\Bar{z}}=\frac{1}{n}\sum_{i=1}^n \mathbf{x}_i^0 +\frac{1}{n}\sum_{i=1}^n \mathbf{y}_i^0$;
%     \item 
%     For $1+n \leq i \leq 2n$ and $t = k\mathcal{B} - 1 + t'$, where $t' = 0, \cdots, \mathcal{B}-1$, 
%     \begin{equation*}
%     \|\mathbf{z}_i^t\| \leq \Gamma \sigma^{k}\sum_{j=1}^{2n}\sum_{m=1}^d |z^0_{jm}|.
%     \end{equation*}
%     and
%     \begin{equation*}
%     \|\mathbf{z}_i^t\| \leq \Gamma (\sigma^{1/\mathcal{B}})^{t-(t'-1) }\sum_{j=1}^{2n}\sum_{m=1}^d |z^0_{jm}|.
%     \end{equation*}
    
% \end{enumerate}
% \end{Theorem1}

%\begin{proof}
As implied by the update \eqref{eq:update_consensus} in Algorithm \ref{alg:A} and the definition of the sparsification operator introduced in Section \ref{sec21}, the mixing matrix and its corresponding product satisfy
	
\begin{equation}\label{z_element}
\begin{aligned}
z_{im}^{t+1}& =\sum_{j=1}^{2n}[\bar{M}^t_m]_{ij} [Q(\z_{j}^t)]_m  + \mathbbm{1}_{\left\{t\mod \mathcal{B} =  \mathcal{B}-1\right\}} \epsilon [F]_{ij} z_{jm}^{\mathcal{B} \lfloor t/\mathcal{B} \rfloor} \\
& = \sum_{j=1}^{2n}[\bar{M}^t_m]_{ij} z^t_{jm} + \mathbbm{1}_{\left\{t\mod \mathcal{B} =  \mathcal{B}-1\right\}} \epsilon [F]_{ij} z_{jm}^{\mathcal{B} \lfloor t/\mathcal{B} \rfloor} = \sum_{j=1}^{2n}[M_m(t:0)]_{ij}z_{jm}^0.
\end{aligned}
\end{equation}
By writing the update recursively and using the fact that $M_m(t:0)$ has column sum equal to $1$, we can represent entries in $\Bar{\z}^t$ as
\begin{equation}\label{zbar_element}
\Bar{z}_m^t =\frac{1}{n}\sum_{j=1}^{2n}z_{jm}^0.
\end{equation}
From equations \eqref{z_element} and \eqref{zbar_element} it follows that 
\begin{equation}
|z_{im}^t -\Bar{z}_m^t| \leq \sum_{j=1}^{2n} |[M_m(t-1:0)]_{ij}-1/n | |z_{jm}^0 |.
\end{equation}
The proof of part (a) is completed by summing $m$ from $1$ to $d$ and applying the results of Lemma \ref{lemma0} while recalling the fact that $\rho(\bar{M}_m(t-1:0))$ has non-zero spectral gap for all $m$, $t$.
Similarly, for $n+1 \leq i \leq 2n$, $
|z_{im}^t| \leq \sum_{j=1}^{2n} |[M_m(t-1:0)]_{ij}  | |z_{jm}^0 |.
$
The proof of part (b) is completed by summing $m$ from $1$ to $d$ and applying the results of Lemma \ref{lemma0}.
%\end{proof}	

\section{Decentralized Optimization Problem}\label{app:B}

\subsection{Proof of Lemma \ref{lemma3}}
	
% \newtheorem*{Lemma2}{Lemma \ref{lemma3}}
% \begin{Lemma2}
% Assumptions \ref{assumption0}, \ref{assumption2}, \ref{assumption3} and \ref{assumption4} imply the following statements:
% \begin{enumerate}[(a)]
%     \item For $1 \leq i \leq n$ and $t = k\mathcal{B} - 1 + t'$, where $t' = 1, \cdots, \mathcal{B}$, it holds that
%     \begin{equation*}
%             \begin{aligned}
%     \|\mathbf{z}_i^{k\mathcal{B}}-\mathbf{\Bar{z}}^{k\mathcal{B}}\| & \leq \Gamma \sigma^{k}\sum_{j=1}^{2n}\sum_{s=1}^d |z^0_{js}| +\sqrt{d}n\Gamma D\sum_{r=1}^{k-1}\sigma^{k-r}\alpha_{r-1} +2\sqrt{d} D\alpha_{k-1},
%     \end{aligned}
%     \end{equation*}
%     and
%     \begin{equation*}
%             \begin{aligned}
%     \|\mathbf{z}_i^t-\mathbf{\Bar{z}}^t\| & \leq \Gamma (\sigma^{1/\mathcal{B}})^{t-(t'-1) } \sum_{j=1}^{2n}\sum_{m=1}^d |z^0_{jm}| +\sqrt{d}n\Gamma D\sum_{r=1}^{\lfloor
%      t/\mathcal{B}\rfloor -1}\sigma^{\lfloor
%      t/\mathcal{B}\rfloor-r}\alpha_{r-1} \\&  +2\sqrt{d} D\alpha_{\lfloor
%      t/\mathcal{B}\rfloor-1}\mathbbm{1}_{t' = 1}.
%     \end{aligned}
%     \end{equation*}
%     \item  For $1+n \leq i \leq 2n$ and $t = k\mathcal{B} - 1 + t'$, where $t' = 1, \cdots, \mathcal{B}$, it holds that
%     \begin{equation*}
%     \begin{aligned}
%     \|\mathbf{z}_i^t\| & \leq \Gamma (\sigma^{1/\mathcal{B}})^{t-(t'-1) } \sum_{j=1}^{2n}\sum_{m=1}^d |z^0_{jm}| 
%      +\sqrt{d}n\Gamma D\sum_{r=1}^{\lfloor
%      t/\mathcal{B}\rfloor -1}\sigma^{\lfloor
%      t/\mathcal{B}\rfloor-r}\alpha_{r-1}.
%     \end{aligned}
%     \end{equation*}
% \end{enumerate}
% \end{Lemma2}

%\begin{proof}
Consider the time step $t=k\mathcal{B}-1$ for some integer $k$ and rewrite the update \eqref{opti_update} as
\begin{equation}
\begin{aligned}
z_{im}^{t+1} &=\sum_{j=1}^{2n}[\bar{M}^t_m]_{ij} [Q(\z_{j}^t)]_m  + \mathbbm{1}_{\left\{t\mod \mathcal{B} = \mathcal{B}-1\right\}} \epsilon [F]_{ij} z_{jm}^{\lfloor t/\mathcal{B} \rfloor} - \mathbbm{1}_{\left\{t\mod \mathcal{B} = \mathcal{B}-1\right\}} \alpha_t g_{im}^{\lfloor t/\mathcal{B} \rfloor} \\
& = \sum_{j=1}^{2n}[\bar{M}^t_m]_{ij} z_{jm}^t + \mathbbm{1}_{\left\{t\mod \mathcal{B} = \mathcal{B}-1\right\}} \epsilon [F]_{ij} z_{jm}^{\lfloor t/\mathcal{B} \rfloor} - \mathbbm{1}_{\left\{t\mod \mathcal{B} = \mathcal{B}-1\right\}} \alpha_t g_{im}^{\lfloor t/\mathcal{B} \rfloor}.
\end{aligned}
\end{equation}
Establishing recursion, we obtain
\begin{equation}
\begin{aligned}
z_{im}^{k\mathcal{B}} & = 
    \sum_{j=1}^{2n}[M_m(k\mathcal{B}-1:0)]_{ij}z_{jm}^0 - \sum_{r=1}^{k-1}\sum_{j=1}^{2n}[M_m((k-1)\mathcal{B}-1:(r-1)\mathcal{B})]_{ij}\alpha_{r-1}g_{jm}^{r-1}\\ &-\alpha_{k-1}g_{im}^{(k-1)\mathcal{B}}.
\end{aligned}
%    \mathbf{z}_i^{k\mathcal{B}} = 
%    \sum_{j=1}^{2n}[M_m(k\mathcal{B}-1:0)]_{ij}z_{jm}^0 - \sum_{r=1}^{k-1}\sum_{j=1}^{2n}[M_m((k-1)\mathcal{B}-1:(r-1)\mathcal{B})]_{ij}\alpha_{r-1}g_{jm}^{r-1}-\alpha_{k-1}g_{i}^{(k-1)\mathcal{B}}
\end{equation}
Using the fact that $M_m(s_2:s_1)$ has column sum equal to $1$ for all $s_2 \geq s_1 \geq 0$, we can represent $\bar{z}_m^{k\mathcal{B}}$ as
\begin{equation}
\begin{aligned}
    \bar{z}_m^{k\mathcal{B}} &= \frac{1}{n}\sum_{j=1}^{2n}z_{jm}^0-\frac{1}{n}\sum_{r=1}^{k-1}\sum_{j=1}^{2n}\alpha_{r-1} g_{jm}^{r-1}-\frac{1}{n}\sum_{j=1}^{n}\alpha_{k-1}g_{jm}^{(k-1)\mathcal{B}}.
\end{aligned}
\end{equation}
By combining the last two expressions,
\begin{equation}
\begin{aligned}
 \|\z_i^{k\mathcal{B}} - \bar{\z}^{k\mathcal{B}} \| 
% \leq \|\sum_{j=1}^{2n}[M_m(k\mathcal{B}-1:0)]_{ij}z_{jm}^0 \\
%& - \sum_{r=1}^{k-1}\sum_{j=1}^{2n}[M_m((k-1)\mathcal{B}-1:(r-1)\mathcal{B})]_{ij}\alpha_{r-1}g_{jm}^{r-1} \alpha_{k-1}g_{i}^{(k-1)\mathcal{B}} 
%\\ &- (\frac{1}{n}\sum_{j=1}^{2n}z_{jm}^0-\frac{1}{n}\sum_{r=1}^{k-1}\sum_{j=1}^{2n}\alpha_{r-1} g_{jm}^{r-1} -\frac{1}{n}\sum_{j=1}^{n}\alpha_{k-1}g_{j}^{(k-1)\mathcal{B}} )
%\|  \\
& \leq \|\sum_{j=1}^{2n}([M_m(k\mathcal{B}-1:0)]_{ij}-\frac{1}{n}) z_{jm}^0 \| \\
&  + \|\sum_{r=1}^{k-1}\sum_{j=1}^{2n}([M_m((k-1)\mathcal{B}-1:(r-1)\mathcal{B})]_{ij}  -\frac{1}{n} )\alpha_{r-1}g_{jm}^{r-1} \| \\
& +  \|\alpha_{k-1}(\mathbf{g}_{i}^{(k-1)\mathcal{B}} - \frac{1}{n}
\sum_{j=1}^{n}\mathbf{g}_{j}^{(k-1)\mathcal{B}} 
) \| .
\end{aligned}
\end{equation}
By using similar techniques to those employed in the proof of Theorem \ref{theorem1}, and invoking the relationship $\|\x \|_2 \leq \|\x \|_1 \leq \sqrt{d}\|\x \|_2$
% \begin{equation*}
% \|\x \|_2 \leq \|\x \|_1 \leq \sqrt{d}\|\x \|_2
% \end{equation*}
for $\x \in \R^d$, we complete the proof of the first inequality in part (a). Proof of the first inequality in part (b) follows the same line of reasoning.
	
To show the correctness of the second inequality in both (a) and (b), we use the fact that for $t \mod \mathcal{B} \neq \mathcal{B}-1$, 
\begin{equation}
z_{im}^{t+1} =\sum_{j=1}^{2n}[\bar{M}^t_m]_{ij} [Q(\z_{j}^t)]_m = \sum_{j=1}^{2n}[\bar{M}^t_m]_{ij} z_{jm}^t
	\end{equation}
	and rewrite $k = \frac{t-(t'-1)}{\mathcal{B}}$. 
This concludes the proof of Lemma \ref{lemma3}.
%\end{proof}

\subsection{Proof of Theorem \ref{theorem3}}
	
% \newtheorem*{Theorem2}{Theorem \ref{theorem3}}
% 	\begin{Theorem2}
% Suppose Assumptions \ref{assumption0}, \ref{assumption2}, \ref{assumption3} and \ref{assumption4} hold. Then, 
% \begin{equation*}
%     \begin{aligned}
%     2\sum_{k=0}^{\infty}\alpha_k (f(\Bar{\mathbf{z}}^{k\mathcal{B}})-f^*) & \leq n\|\Bar{\mathbf{z}}^0 -\mathbf{x}^*\| + nD'^2\sum_{k=0}^{\infty}\alpha_k^2  +\frac{4D'}{n}\sum_{i=1}^n \sum_{k=0}^{\infty} \alpha_k \| \mathbf{z}_i^{k\mathcal{B}}-\Bar{\mathbf{z}}^{k\mathcal{B}}\|.
% \end{aligned}  
% \end{equation*}

% \end{Theorem2}
% \begin{proof}
Recall the update \eqref{opti_update}
%\begin{equation*}
%\begin{aligned}
% z_{im}^{t+1} & =\sum_{j=1}^{2n}[\bar{M}^t_m]_{ij} [Q(\z_{j}^t)]_m + \mathbbm{1}_{\left\{t\mod \mathcal{B} = \mathcal{B}-1\right\}} \epsilon [F]_{ij} z_{jm}^{\mathcal{B} \lfloor t/\mathcal{B} \rfloor} \\&
% - \mathbbm{1}_{\left\{t\mod\mathcal{B} = \mathcal{B}-1\right\}} \alpha_{\lfloor t/\mathcal{B} \rfloor} g_{im}^{\mathcal{B} \lfloor t/\mathcal{B} \rfloor},
%\end{aligned}
%\end{equation*}
and note that
$
\Bar{\z}^{(k+1)\mathcal{B}}=\Bar{\z}^{k\mathcal{B}}-\frac{\alpha_t}{n}\sum_{i=1}^n \nabla f_i(\z_i^{k\mathcal{B}}).
$
We thus have that
\begin{equation}
\begin{aligned}
\|\Bar{\z}^{k\mathcal{B}+k}-\x^* \|^2 = \|\frac{\alpha_k}{n}\sum_{i=1}^n \nabla f_i(\z_i^{k\mathcal{B}}) \|^2 +\|\Bar{\z}^{k\mathcal{B}}-\x^* \|^2-\frac{2\alpha_k}{n}\sum_{i=1}^n \langle \Bar{\z}^{k\mathcal{B}}-\x^*, \nabla f_i(\z_i^{k\mathcal{B}}) \rangle.
\end{aligned}
\end{equation}
On the other hand,
\begin{equation}
\begin{aligned}
\|\Bar{\z}^{t}-\x^* \|^2 %& = \|\Bar{\z}^{t-1}-\x^* \|^2 \\
= \|\Bar{\z}^{k\mathcal{B}}-\x^* \|^2+\|\frac{\alpha_k}{n}\sum_{i=1}^n \nabla f_i(\z_i^{k\mathcal{B}}) \|^2  -\frac{2\alpha_k}{n}\sum_{i=1}^n \langle \Bar{\z}^{k\mathcal{B}}-\x^*, \nabla f_i(\z_i^{k\mathcal{B}}) \rangle
\end{aligned}
\end{equation}
for % $t \mod{\mathcal{B}} \neq 0$ and 
$t = k\mathcal{B}-1+t'$ and $t' = 1, \cdots, \mathcal{B}-1$. 
Therefore, 
\begin{equation}
	\begin{aligned}
	\|\Bar{\z}^{k\mathcal{B}+k}-\x^* \|^2 = \|\Bar{\z}^{k\mathcal{B}}-\x^* \|^2+\|\frac{\alpha_k}{n}\sum_{i=1}^n \nabla f_i(\z_i^{k\mathcal{B}}) \|^2  -\frac{2\alpha_k}{n}\sum_{i=1}^n \langle \Bar{\z}^{k\mathcal{B}}-\x^*, \nabla f_i(\z_i^{k\mathcal{B}})  \rangle.
	\end{aligned}
\end{equation}
Since $|g_{im}| \leq D$ and $D'=\sqrt{d}D$, and by invoking the convexity of $f$,
\begin{equation}
\begin{aligned}
\langle \Bar{\z}^{k\mathcal{B}}-\x^*, \nabla f_i(\z_i^{k\mathcal{B}})  \rangle  & = \langle \Bar{\z}^{k\mathcal{B}}-\z_i^{k\mathcal{B}}, \nabla f_i(\z_i^{k\mathcal{B}})  \rangle+  \langle \z_i^{k\mathcal{B}}-\x^*, \nabla f_i(\z_i^{k\mathcal{B}})  \rangle \\
%	& \geq \langle \Bar{\z}^{k\mathcal{B}}-\z_i^{k\mathcal{B}}, \nabla f_i(\z_i^{k\mathcal{B}}) \rangle +f_i(\z_i^{k\mathcal{B}})-f_i(\x^*) \\
	& \geq -D'\|\Bar{\z}^{k\mathcal{B}}-\z_i^{k\mathcal{B}} \|+f_i(\z_i^{k\mathcal{B}})-f_i(\Bar{\z}^{k\mathcal{B}}) +f_i(\Bar{\z}^{k\mathcal{B}})-f_i(\x^*)  \\
	& \geq -2D'\|\Bar{\z}^{k\mathcal{B}}-\z_i^{k\mathcal{B}} \|+f_i(\Bar{\z}^k\mathcal{B})-f_i(\x^*).
\end{aligned}
\end{equation}

Rearranging the terms above and summing from $t=0$ to $\infty$ completes the proof. 
%\end{proof}

\subsection{Proof of Theorem \ref{theorem4}}

% \newtheorem*{Theorem3}{Theorem \ref{theorem4}}
% \begin{Theorem3}
% Suppose Assumptions \ref{assumption0}, \ref{assumption2}, \ref{assumption3} and \ref{assumption4} hold. For the stepsize $\alpha_t = O(1/\sqrt{t})$, Algorithm \ref{alg:B} attains the convergence rate $O(\frac{\log(T)}{\sqrt{T}})$. 
% \end{Theorem3}

% \begin{proof}
First we derive an intermediate proposition.
\begin{adjustwidth}{0.5cm}{0cm}\qquad
\begin{proposition}
For each $m$ and $ k$, the following inequalities hold:
\begin{enumerate}[(a)]
\item For $1 \leq i \leq n$, $\sum_{k=0}^{\infty} \alpha_k |z_{im}^{k\mathcal{B} }-\Bar{z}_m^{k\mathcal{B}}| < \infty$.
\item For $n+1 \leq i \leq 2n$, $\sum_{k=0}^{\infty} \alpha_k |z_{im}^{k\mathcal{B}}| < \infty$.
\end{enumerate}
\end{proposition}
\begin{proof}
Using the result of Lemma \ref{lemma3}(a), for $1 \leq i \leq n$, \begin{equation}
	\begin{aligned}
	\sum_{k=1}^T\alpha_k \|\z_i^{k\mathcal{B}}-\Bar{\z}^{k\mathcal{B}} \| & \leq \Gamma (\sum_{j=1}^{2n}\sum_{s=1}^d|z^0_{js}|)\sum_{k=1}^T \alpha_k \sigma^k 
	+\sqrt{d} n\Gamma D\sum_{k=1}^T\sum_{r=1}^{k-1}\sigma^{t-r}\alpha_k \alpha_{r-1}\\& +2\sqrt{d}D \sum_{k=0}^{T-1}\alpha_k^2.
	\end{aligned}
	\end{equation} 
	Applying inequality $ab \leq \frac{1}{2}(a+b)^2, a, b \in \mathcal{R}$,
	\begin{equation}
	\sum_{k=1}^T \alpha_k \sigma^k \leq \frac{1}{2}\sum_{k=1}^T (\alpha_k^2+ \sigma^{2k}) \leq \frac{1}{2}\sum_{k=1}^T \alpha_k^2 + \frac{1}{1-\sigma^2}
	\end{equation}
	\begin{equation}
	\begin{aligned}
	\sum_{k=1}^T\sum_{r=1}^{k-1}\sigma^{k-r}\alpha_k \alpha_{r-1} \leq \frac{1}{2}\sum_{k=1}^T\alpha_k^2 \sum_{r=1}^{r-1} \sigma^{k-r}  + \frac{1}{2}\sum_{r=1}^{T-1}\alpha_{r-1}^2 \sum_{k=r+1}^{T} \sigma^{k-r} \leq \frac{1}{1-\sigma}\sum_{k=1}^T \alpha_k.
	\end{aligned}
	\end{equation}
	Using the assumption that the step size satisfies $\sum_{k=0}^{\infty} \alpha_t^2 < \infty$ as $T \to \infty$, we complete the proof of part (a).
	The same techniques can be used to prove part (b).
\end{proof}
\end{adjustwidth}
We can now continue the proof of the stated convergence rate. Since the mixing matrices have columns that sum up to one we have $\bar{z}^{k\mathcal{B}+t'-1} = \bar{k\mathcal{B}},$
% \begin{equation}
%     \bar{z}^{k\mathcal{B}+t'-1} = \bar{k\mathcal{B}}
% \end{equation}
for all $t' = 1, \cdots, \mathcal{B}$. 

In the following step, we consider $t = k\mathcal{B}$ for some integer $k \geq 0$. Defining $f_{\min}:=\mathrm{min}_t f(\Bar{\mathbf{z}}^t)$, we have
\begin{equation}\label{eq:temp:proof}
\begin{aligned}
(f_{\min}-f^*)\sum_{t=0}^T\alpha_t &\leq \sum_{t=0}^T\alpha_t(f(\Bar{\mathbf{z}}^t)-f^* )\leq C_1+C_2\sum_{t=0}^T\alpha_t^2,
\end{aligned}
\end{equation}
where 
\begin{equation}
    C_1 =\frac{n}{2}(\|\Bar{\mathbf{z}}^0-\mathbf{x}^*\|^2-\|\Bar{\mathbf{z}}_{T+1}-\mathbf{x}^* \|^2) +D'\Gamma \sum_{j=1}^{2n}\frac{\|\mathbf{z}_j^0\|}{1-\sigma^2},
\end{equation}
\begin{equation}
C_2=\frac{nD'^2}{2}+4D'^2+D'\Gamma \sum_{j=1}^{2n}\|\mathbf{z}_j^0\|+\frac{2D'^2\Gamma}{1-\sigma}.
\end{equation}
Note that we can express \eqref{eq:temp:proof} equivalently as
\begin{equation}\label{eq:temp:proof2}
(f_{\min}-f^*)\leq \frac{C_1}{\sum_{t=0}^T\alpha_t}+\frac{C_2 \sum_{t=0}^T\alpha_t^2}{\sum_{t=0}^T\alpha_t}.
\end{equation}
Now, by recalling the statement of Assumption \ref{lemma3}, we have that $\alpha_t=o(1/\sqrt{t})$. If we select the schedule of stepsizes according to $\alpha_t=1/\sqrt{t}$, the two terms on the right hand side of \eqref{eq:temp:proof2} satisfies 
\begin{equation}
   \frac{C_1}{\sum_{t=0}^T\alpha_t} = C_1 \frac{1/2}{\sqrt{T}-1}=\O(\frac{1}{\sqrt{T}}),
    \frac{C_2 \sum_{t=0}^T\alpha_t^2}{\sum_{t=0}^T\alpha_t}=C_2 \frac{\mathrm{ln}T}{2(\sqrt{T}-1)}=\O(\frac{\mathrm{ln}T}{\sqrt{T}}). 
\end{equation}
This completes the proof.
%\end{proof}

% \begin{comment}
% Upon defining $f_{\min}:=\mathrm{min}_t f(\Bar{\mathbf{z}}^t)$, we have
% \begin{equation}\label{eq:temp:proof}
% (f_{\min}-f^*)\sum_{t=0}^T\alpha_t \leq \sum_{t=0}^T\alpha_t(f(\Bar{\mathbf{z}}^t)-f^* )
% \leq C_1+C_2\sum_{t=0}^T\alpha_t^2,
% \end{equation}
% where 
% \begin{equation}
% \begin{aligned}
% C_1&=\frac{n}{2}(\|\Bar{\mathbf{z}}^0-\mathbf{x}^*\|^2-\|\Bar{\mathbf{z}}_{T+1}-\mathbf{x}^* \|^2)\\
% &\qquad+D'\Gamma \sum_{j=1}^{2n}\frac{\|\mathbf{z}_j^0\|}{1-\sigma^2},
% \end{aligned}
% \end{equation}
% and
% \begin{equation}
% C_2=\frac{nD'^2}{2}+4D'^2+D'\Gamma \sum_{j=1}^{2n}\|\mathbf{z}_j^0\|+\frac{2D'^2\Gamma}{1-\sigma}.
% \end{equation}
% Note that we can express \eqref{eq:temp:proof} equivalently as
% \begin{equation}\label{eq:temp:proof2}
% (f_{\min}-f^*)\leq \frac{C_1}{\sum_{t=0}^T\alpha_t}+\frac{C_2 \sum_{t=0}^T\alpha_t^2}{\sum_{t=0}^T\alpha_t}.
% \end{equation}
% Now, by recalling the statement of Assumption \ref{lemma3}, we have that $\alpha_t=o(1/\sqrt{t})$. If we select the schedule of stepsizes according to $\alpha_t=1/\sqrt{t}$, the first term on the right hand side of \eqref{eq:temp:proof2} satisfies 
% \begin{equation}
%   \frac{C_1}{\sum_{t=0}^T\alpha_t} = C_1 \frac{1/2}{\sqrt{T}-1}=\O(\frac{1}{\sqrt{T}}),
% \end{equation}
% while for the second term it holds that
% \begin{equation}
%     \frac{C_2 \sum_{t=0}^T\alpha_t^2}{\sum_{t=0}^T\alpha_t}=C_2 \frac{\mathrm{ln}T}{2(\sqrt{T}-1)}=\O(\frac{\mathrm{ln}T}{\sqrt{T}}). 
% \end{equation}
% \end{comment}
	%%%%%%%%%%%%%%%%%%%%%%%%%%%%%%%%%%%%%%%
	%%%%%%%%%%%%%%%%%%%%%%%%%%%%%%%%%%%%%%%
	%\newpage
	\section{ Communication-Sparsification on Random Graphs}\label{app:C}
	In this section, we discuss the effect of compression rate, i.e. $k/d$, on the spectral gap in jointly-connected graphs. 
	First, we consider the special case where the graph is connected at each time step, which leads to the mixing matrix in \eqref{matrixdef},
% 	\begin{equation*}%\label{matrixdefCappendix}
% 	M_m^t=\left[\begin{matrix}
% 	A_m^t & \epsilon I \\
% 	I-A_m^t & B_m^t-\epsilon I \\
% 	\end{matrix}
% 	\right],
% 	\end{equation*}
	under the assumption that the communication links among the agents in the network are generated according to the  Erdős–Rényi model \cite{erdos1959random}. It will be convenient to review some facts and state the following definition. 
	\begin{definition}
		[\cite{erdos1959random}]
		A random graph $\G(n,p)$ with $n$ nodes is an Erdős–Rényi graph if every edge is included in the graph with probability $0<p<1$ independent from every other edge.
	\end{definition}
	It is easy to see that the expected degree of each node is $\mathrm{deg} = (n-1)p \simeq np$. 

	A directed Erdős–Rényi graph can be thought of as a union of two undirected Erdős–Rényi graphs $\G_1(n,\mathrm{in\_deg}/(n-1))$ and $\G_2(n,\mathrm{out\_deg}/(n-1))$. Let $W = \bar{W}/|\lambda_1(\bar{W})|$ denote the normalized adjacency matrix of a directed Erdős–Rényi graph, where $\bar{W}$ is the unnormalized adjacency matrix and $\lambda_1(\bar{W})$ is the largest eigenvalue of $\bar{W}$. Since $W$ and $W^\top$ have identical eigen-space and both have $1$ as the largest eigenvalue, $W$ and the symmetric matrix $S = \frac{W+W^\top}{2}$ have similar spectral gaps. Note that $S$ itself can be thought of as the adjacency matrix of an undirected Erdős–Rényi graph $\G_1(n,\bar{d}/(n-1))$, where $\bar{d} = \frac{\mathrm{in\_deg}+\mathrm{out\_deg}}{2}$. Therefore, in order to establish our results, we concentrate on studying the impact of the compression rate on the spectral gap of the mixing matrix $M_m^t$
	given that matrices $A_m^t$ and $B_m^t$ correspond to undirected Erdős–Rényi graphs.
	
	Erdős–Rényi random graphs are known for entailing sharp transitions in their monotone graph properties, as formalized by the following theorem.
	\begin{theorem}
		[\cite{erdos1959random,benaych2019largest}] Let $p = \frac{g(n)}{n}$ be the edge probability of an Erdős–Rényi random graph $\G(n,p)$ with normalized adjacency matrix $W$.
		\begin{enumerate}[(a)]
			\item If $g(n) <1$, then $\G(n,p)$ will almost surely be disconnected.
			\item If $g(n) >1$, then $\G(n,p)$ will almost surely be connected and $|\lambda_2(W)|<2/\sqrt{g(n)}$.
		\end{enumerate}
	\end{theorem}
	Since message-sparsification can be thought of as adversely affecting network connectivity and since the probability of sparsifying a specific entry
	is $1-k/d$, we define effective edge probability for a network with sparsified messages as $q = p(1-(1-k/d)^2)$. Having $g(n) > \frac{1}{1-(1-k/d)^2}$ ensures that after sparsification the graph remains connected almost surely at each time $t$ and thus Assumption 1 in the main paper holds.
	
	Next, we establish a relation between the spectral gap of $M_m^t$ and the compression rate $k/d$. Note that since $\Bar{M}_m^t$ in \eqref{matrixdefbar}
% 	\begin{equation*}%\label{matrixdefM}
% 	\Bar{M}_m^t=\left[\begin{matrix}
% 	A_m^t & \mathbf{0} \\
% 	I-A_m^t & B_m^t \\
% 	\end{matrix}
% 	\right]
% 	\end{equation*}
	is block (lower) triangular, its spectrum is a union of the spectrum of $A_m^t$ and $B_m^t$. However, since $g(n) > \frac{1}{1-(1-k/d)^2}$, and $A_m^t$ and $B_m^t$ are normalized (i.e. their largest eigenvalue is 1), it holds that 
	\begin{equation}
	|\lambda_3(\Bar{M}_m^t)|< \frac{2}{\sqrt{g(n)(1-(1-k/d)^2)}} \leq \sqrt{\frac{4d}{kg(n)}}
	\end{equation}
	almost surely. Now, following the proof of Theorem \ref{theorem1} in \cite{cai2011average} we can establish that $\sigma \leq 1-\alpha n \epsilon$, where $\alpha >0$ is a positive constant, $\epsilon \in (0, \bar{\gamma})$ with  $\bar{\gamma} = \frac{1}{(20+8n)^n}(1-\sqrt{\frac{4d}{kg(n)}})^n$, and 
	$\sigma = \max_{C \in \mathcal{U}_M^t} |\lambda_2(C)|<1$; here $\mathcal{U}_M^t$ denotes the finite set of all possible mixing matrices at time $t$. Thus, there exists a $0<\beta <1$ such that 
	$
	\sigma = 1-\frac{\alpha\beta n}{(20+8n)^n}(1-n\sqrt{\frac{4d}{kg(n)}} )
	$
	almost surely.
	
	Let us now turn attention to $\mathcal{B}$-jointly-connected graphs.
	%Recall that for two Erdos-Renyi random graphs, $\G(n, p_1)$ and $\G(n, p_2)$, the union graph $\G = \G(n, p_1) \bigcup \G(n, p_2)$ is still an Erdos-Renyi random graph with probability parameter $p = p_1+p_2-p_1p_2$. 
	The possibility of sparsifying a specific entry over $\mathcal{B}$ time steps is $(1-k/d)^{\mathcal{B}}$. Thus we can derive the edge probability in a network with sparsified messages over $\mathcal{B}$ time steps as $q = p(1-(1-k/d)^{2\mathcal{B}} )$. Following the same technique used above, we have that
	\begin{equation}
	\begin{aligned} |\lambda_3(\bar{M}_m((k+1)\mathcal{B}-1:k\mathcal{B}))| 
	<  \frac{2}{\sqrt{g(n)(1-(1-k/d)^{2\mathcal{B}} )}} 
	 \leq 
	\sqrt{\frac{4}{(1-(1-k/d)^{\mathcal{B}})g(n)}}
	\end{aligned}
	\end{equation}
	and
	$
	    \sigma = 1-\frac{\alpha\beta n}{(20+8n)^n}(1-n\sqrt{\frac{4}{(1-(1-k/d)^{\mathcal{B}})g(n)}} ).
	$
	%%%%%%%%%%%%%%%%%%%%%%%%%%%
	%%%%%%%%%%%%%%%%%%%%%%%%%%%%
\begin{figure*}[t]
	\centering
	\minipage[t]{1\linewidth}
	\begin{subfigure}[t]{.49\linewidth}
		\includegraphics[width=\textwidth]{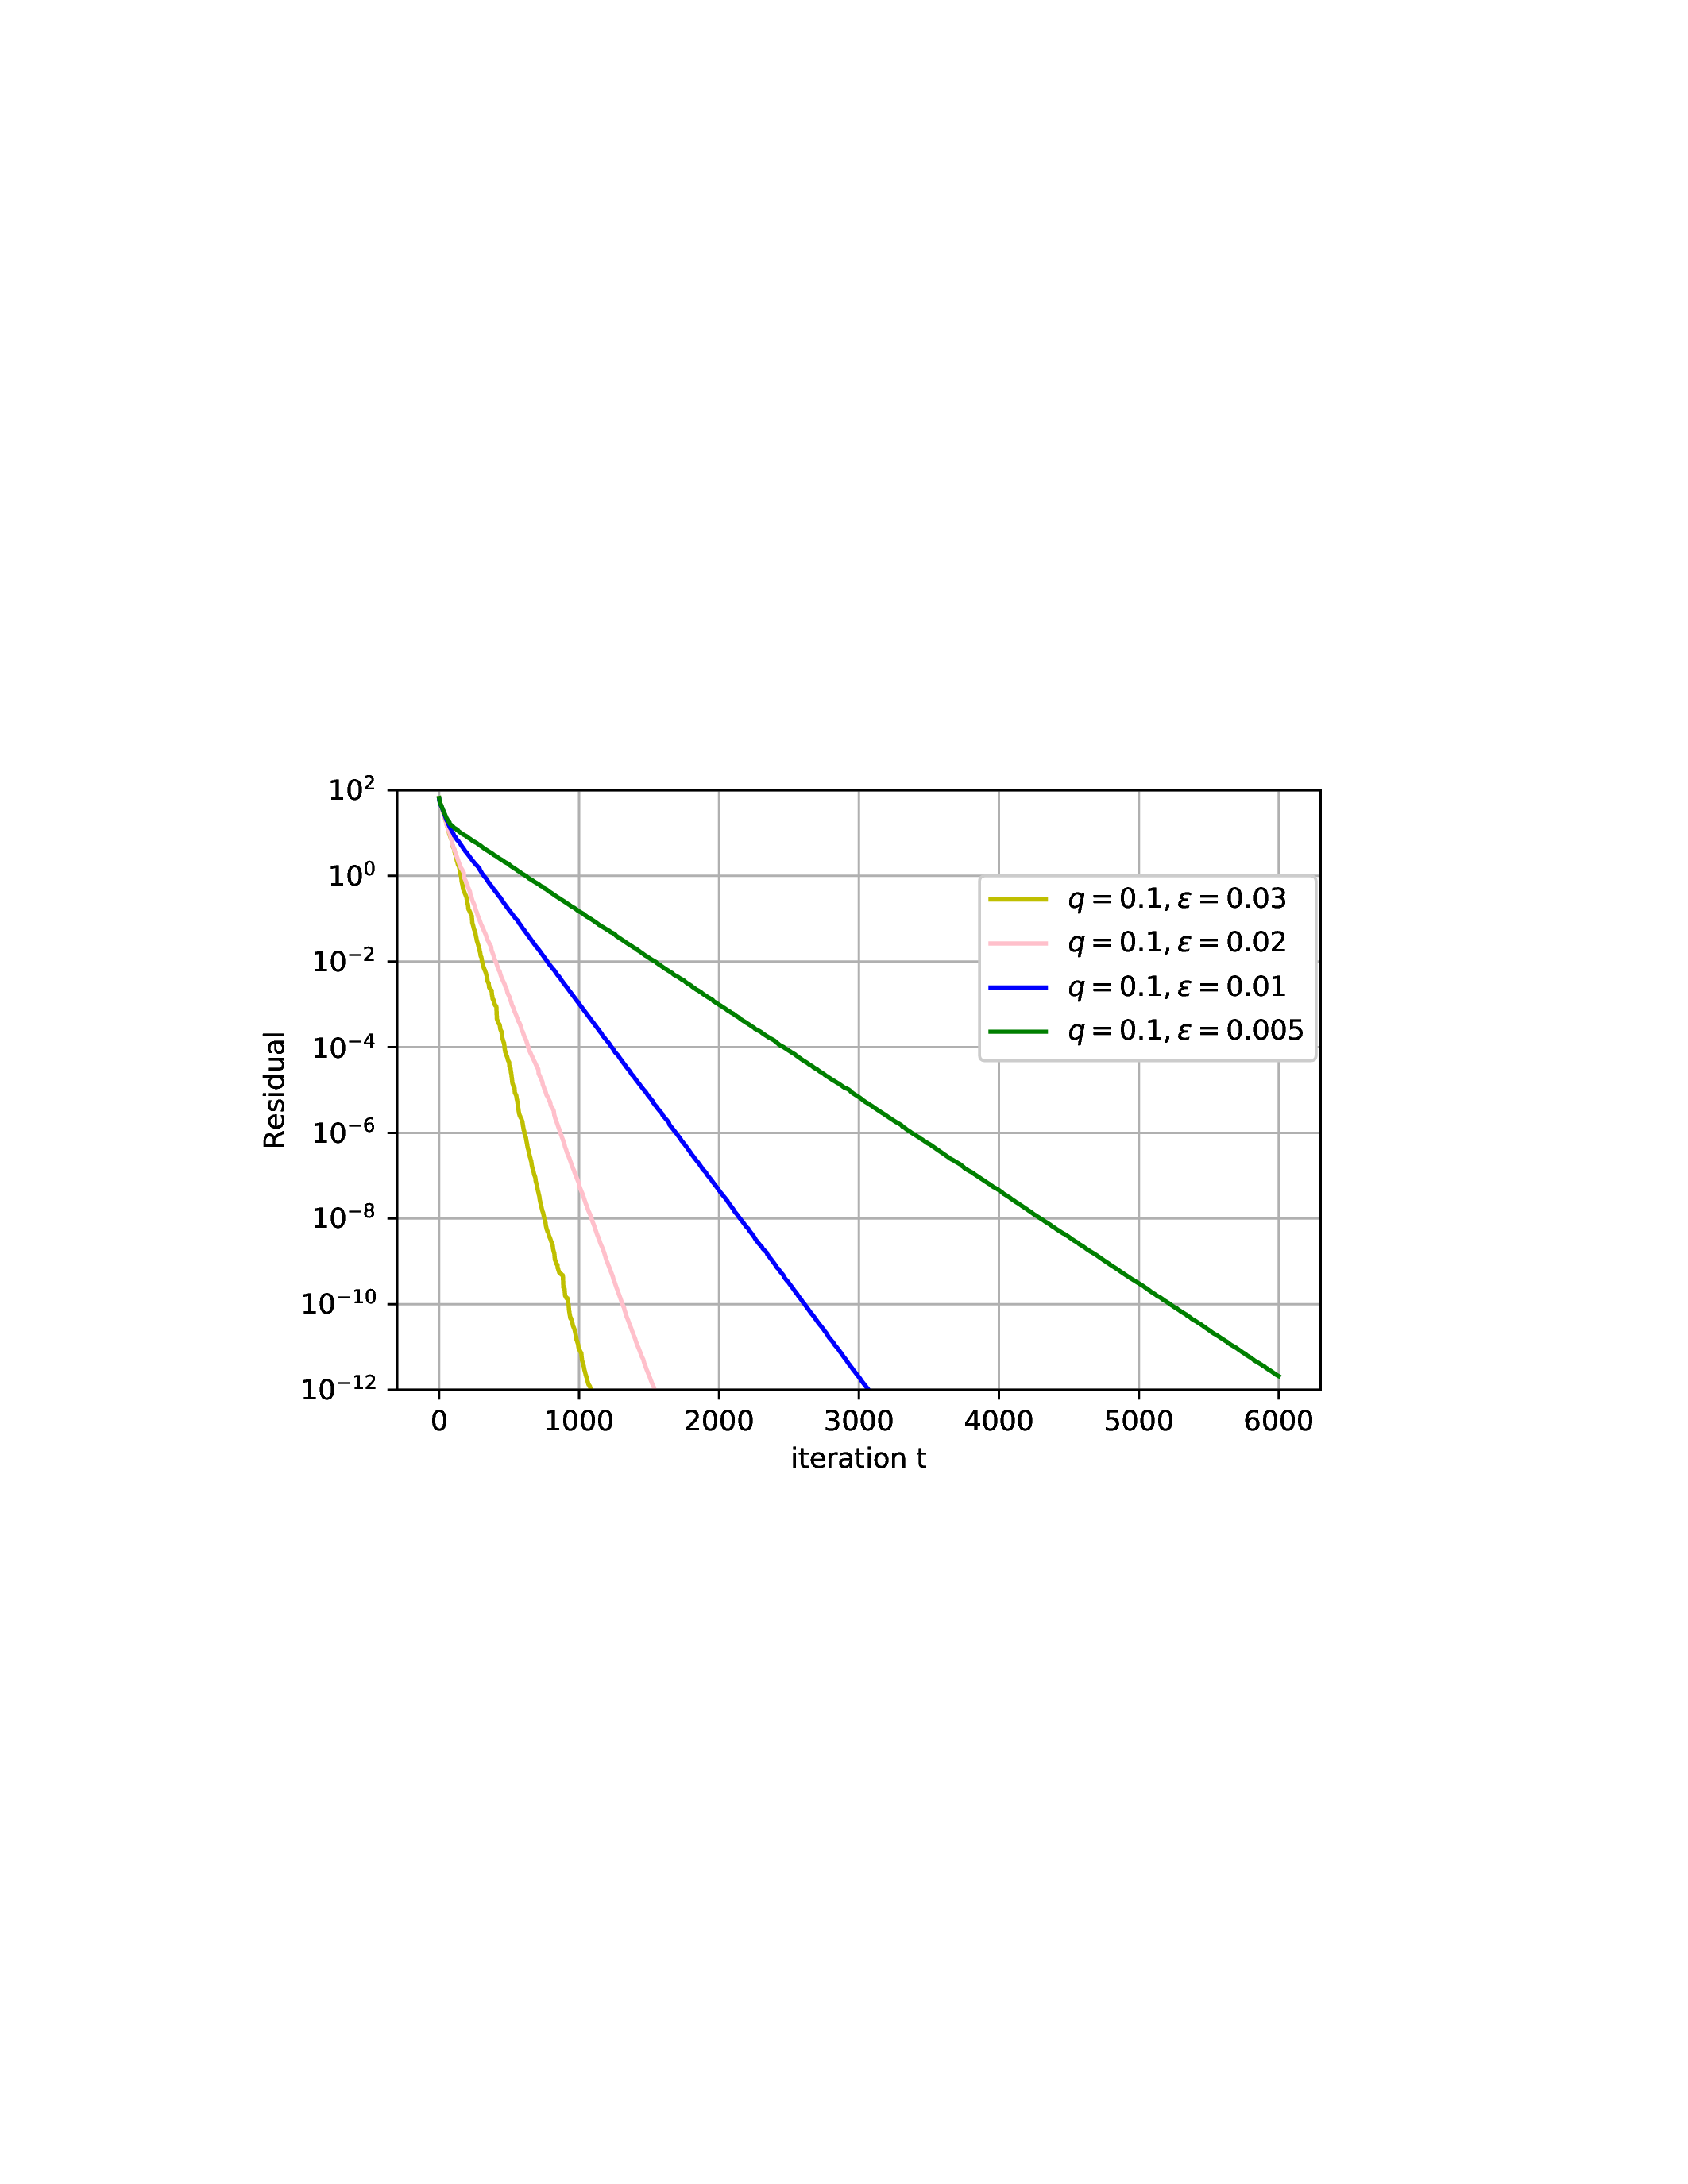}
		\caption{\footnotesize  Average consensus model}
	\end{subfigure}
	\begin{subfigure}[t]{.49\linewidth}
		\includegraphics[width=\linewidth]{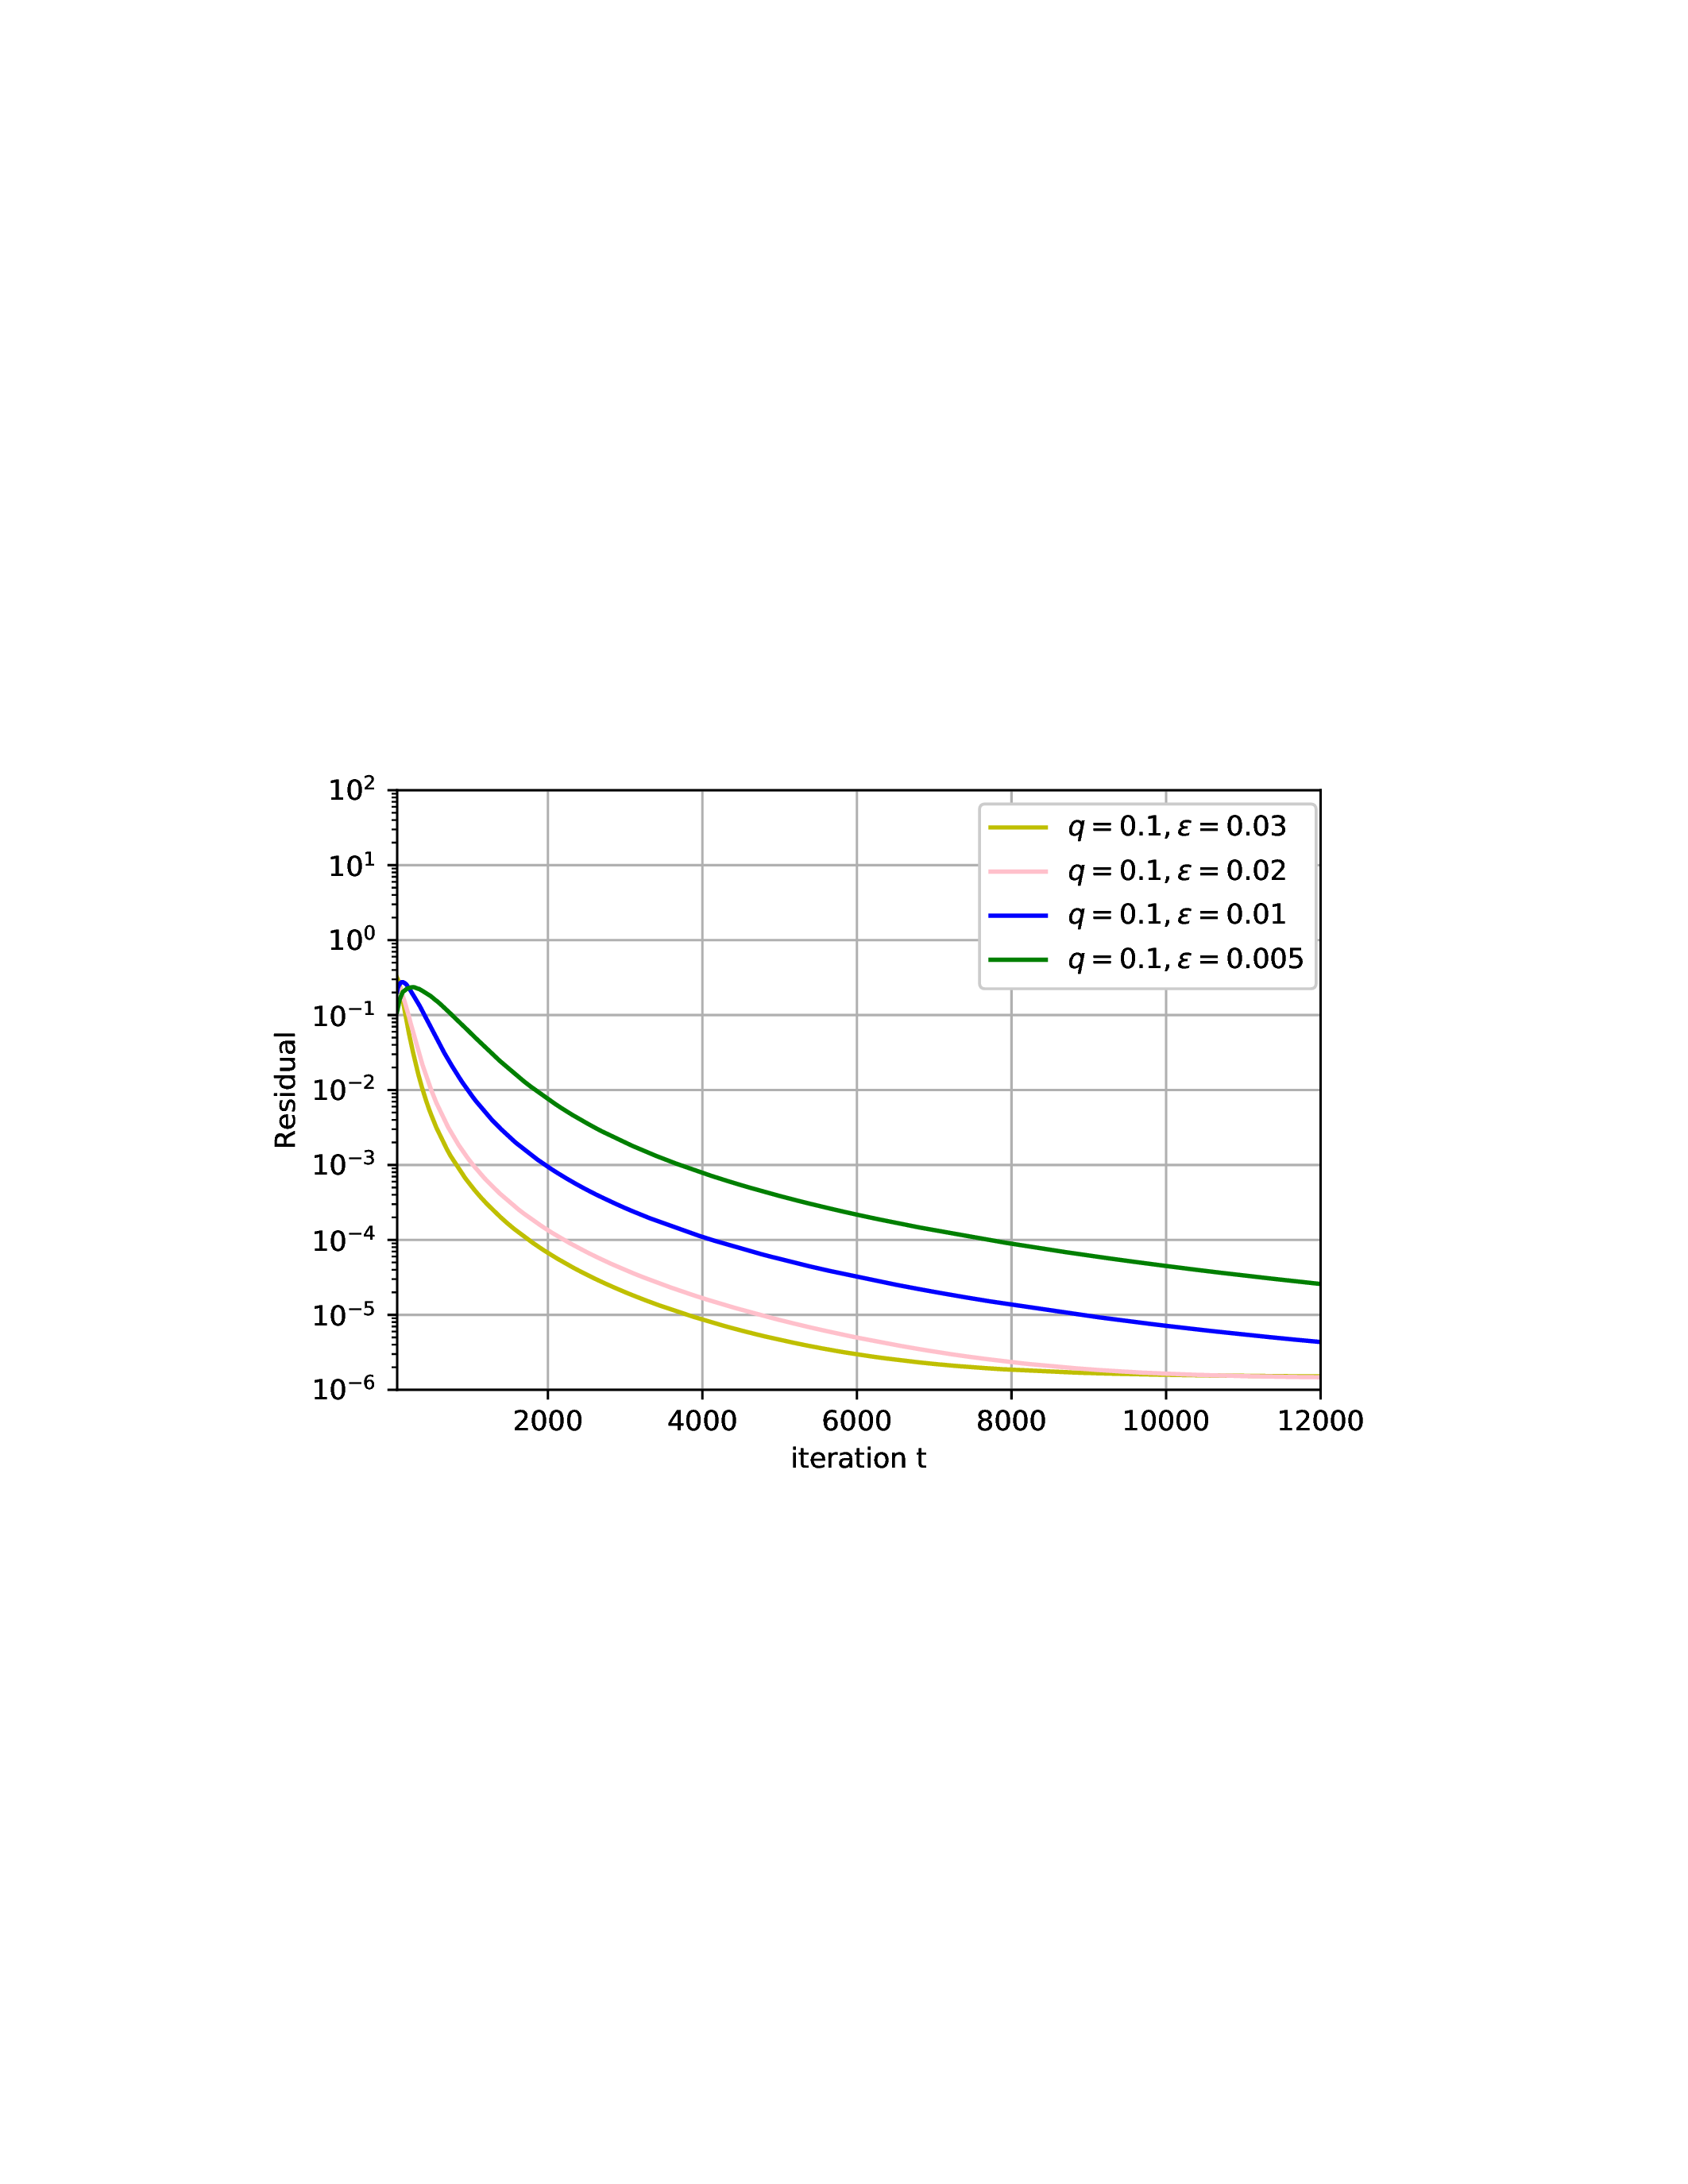}
		\caption{\footnotesize Linear regression model}
	\end{subfigure}
	\caption{Experimental results on varying the value of $\epsilon$.}
	\label{fig:epsilon}
	\endminipage 
		\vspace{-0.4cm}
    \end{figure*}

    \begin{figure*}[t]
	\centering
	\minipage[t]{1\linewidth}
	\begin{subfigure}[t]{.49\linewidth}
		\includegraphics[width=\textwidth]{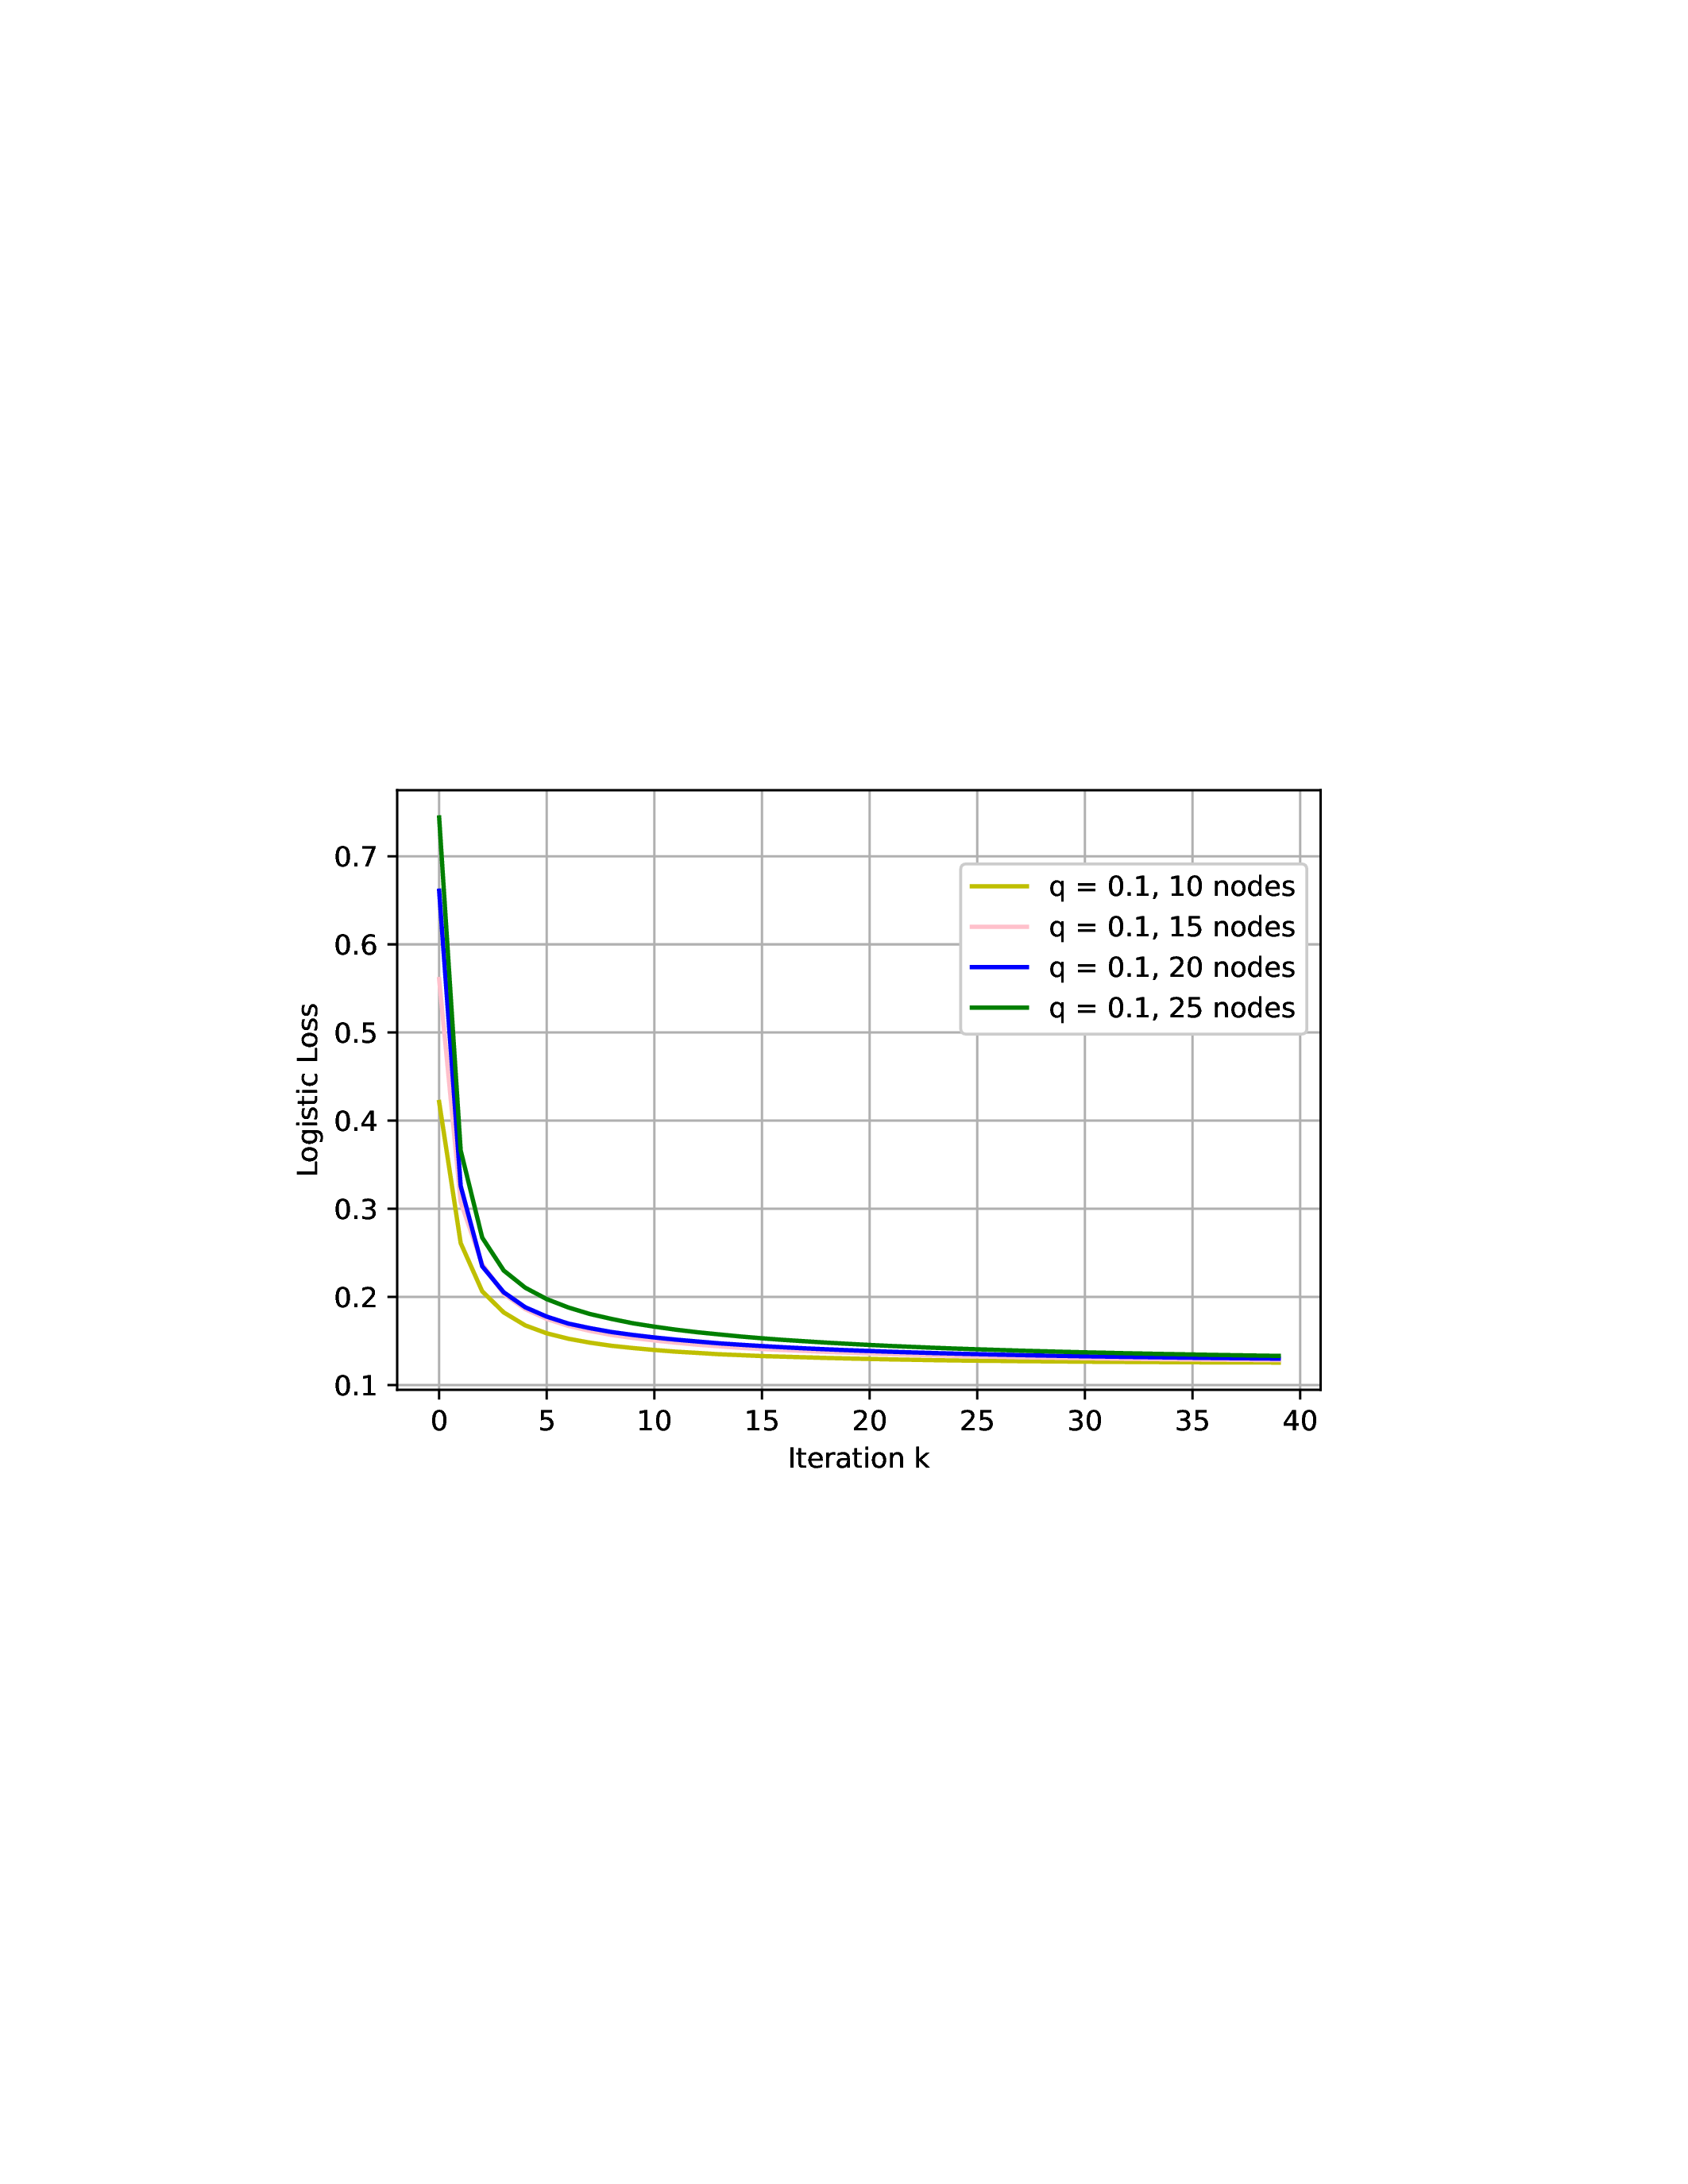}
		\caption{\footnotesize  Loss}
	\end{subfigure}
	\begin{subfigure}[t]{.49\linewidth}
		\includegraphics[width=\linewidth]{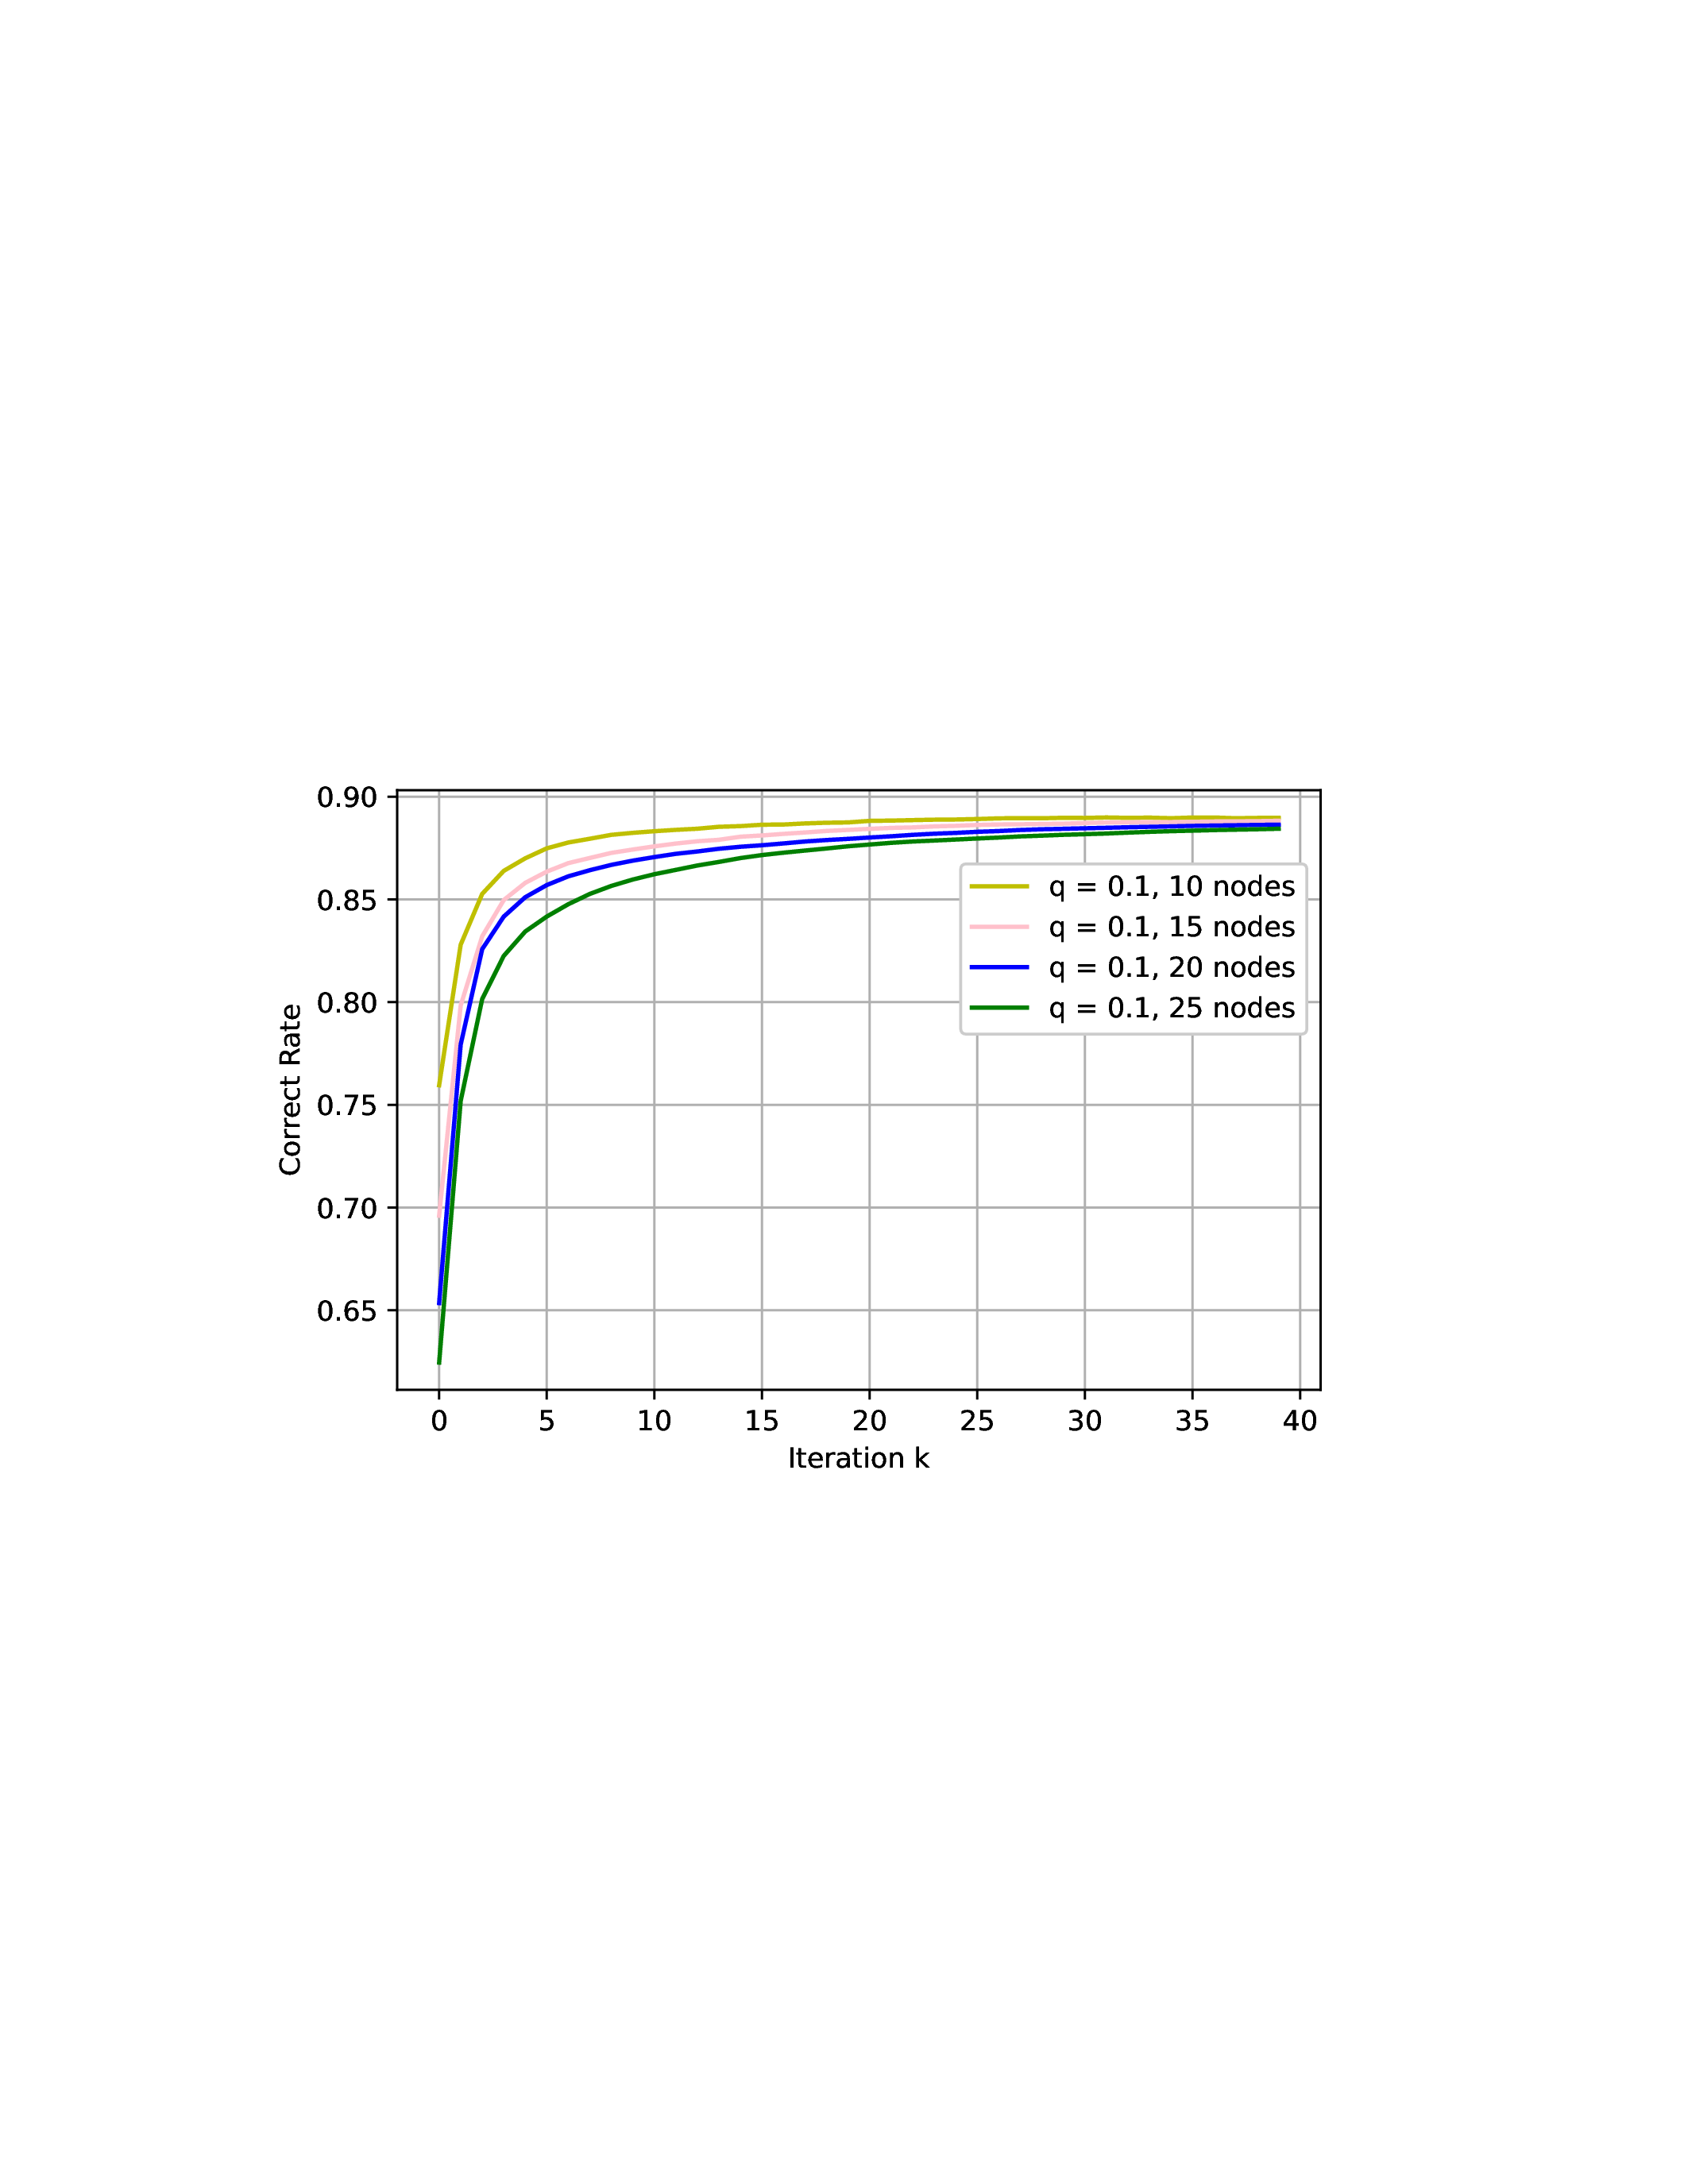}
		\caption{\footnotesize Correct rate}
	\end{subfigure}
	\caption{Experimental results on optimization algorithm over time-varying directed network: different sizes of network.}
	\label{fig:logi_nodes}
	\endminipage 
		\vspace{-0.6cm}
    \end{figure*}	
	%%%%%%%%%%%%%%%%%%%%%%%%%%%%%%%%%%%%%%%
	%%%%%%%%%%%%%%%%%%%%%%%%%%%%%%%%%%%%%%%
	%\newpage
\section{Further Experimental Results}\label{app:D}
\subsection{Varying the values of perturbation parameters}
In this section, we expand on the experiments presented in the main paper by considering effects of varying parameter $\epsilon$; recall that $\epsilon$ is a parameter characterizing the perturbation of the mixing matrix from the original $\Bar{M}$. Please see Figure \ref{fig:epsilon} (a) for the results of average consensus experiments and Figure  \ref{fig:epsilon} (b) for the results of linear regression experiments. We consider $4$ levels of perturbations -- $\epsilon = 0.1$, $0.05$, $0.02$, $0.01$ -- and show the corresponding convergence results. Other parameters are set to the same values as in the main paper. 
	
%	First we consider sparsification rate no more than $50\%$. We show experimental results when the sparsification rates are $30\%$ and $20\%$. Here we are comparing to a fully connected graph, i.e., sparsification rate $20\%$ means each node communicates each of its update parameters to $1$ neighboring node and there are $2$ out of $10$ nodes knowing this update. 
In the main paper, we argued that the proposed algorithms achieve claimed convergence properties for a range of $\epsilon$; this range is further specified for a family of graphs in Appendix \ref{app:A}. For the simulations presented here, we choose a relatively large $\epsilon$ to accelerate the convergence. In particular, we set $\epsilon \leq 0.1$; given the choice of other parameters, such $\epsilon$ ensures non-zero spectral gap and guarantees the claimed convergence properties.

In the average consensus problem, as Figure \ref{fig:epsilon} (a) shows, Algorithm \ref{alg:A} achieves convergence linear in $t$. The convergence rate decreases as we reduce the value of $\epsilon$. In the linear regression problem, as Figures \ref{fig:epsilon} (b) shows, convergence of Algorithm \ref{alg:B} is slowed down as $\epsilon$ is reduced.
	% Comparing bits of communication to push-sum algorithm
	
\subsection{Varying the graph size}
	
We further studied the performance of the proposed algorithms in applications to graphs of varied size, i.e., experimented with the number of network nodes; the results are shown in Figure \ref{fig:logi_nodes}. In the logistic regression problem, the total number of data points is fixed and therefore the number of local data points is inversely proportional to the number of nodes in the network. For each model, we consider $4$ different sizes of network; other parameter settings are kept the same as in the main paper.
	
For this experiment, we consider two metrics: logistic loss and correct classification rate (accuracy). These metrics exhibit the same convergence behavior as the network size is varied. In particular, we observe that in larger networks Algorithm \ref{alg:B} converges slower but still reaches the optimal solution. 

\subsection{Quantized D-DGD and subgradient-push algorithms}
%	As mentioned in the footnote of the main paper, we attempt imposing direct sparsification into the ideas of D-DGD and push-sum algorithm. Since the consensus state cannot be achieved, as shown in figure \ref{fig:cons_unw}, the modification on previous algorithms cannot reach convergence.
    
As stated in Section \ref{simulation_sec} of the paper, in our benchmarking studies of Algorithm \ref{alg:A} and Algorithm \ref{alg:B} we consider two quantized versions of the push-sum and subgradient-push algorithms, respectively. 

%Since the consensus state cannot be achieved in the time-varying directed networks, they cannot reach convergence.
    
The first benchmarking quantization scheme is the quantized subgradient-push algorithm, referred to as Q-Grad-Push in Section \ref{simulation_sec} \cite{nedic2014distributed}.  This scheme is implemented by applying quantization to the vanilla subgradient-push algorithm in the following way: each node quantizes entries in the local state vector $x(t)$ according to given quantization levels, and communicates the compressed vectors to its neighboring nodes, i.e.,
    \begin{align*}
	&\mathbf{w}(t+1) =A(t)Q(\x(t)), \qquad
	y(t+1) =A(t)y(t) \\
	&\z_i(t+1) = \frac{\mathbf{w}_i(t+1)}{y_i(t+1)}, \qquad
	\x(t+1) = \mathbf{w} (t+1) - \alpha_{t+1}\nabla F(\z(t+1)),
	\end{align*}
where $A(t)$ denotes the mixing matrix at current time. The quantized push-sum algorithm (referred to as Q-Push-Sum in Section \ref{simulation_sec}) follows the same procedure as Q-Grad-Push expect for inclusion of a gradient term.
The push-sum and subgradient-push algorithms without quantization converge to the optimal solution when deployed over time-varying directed networks but no convergence is guaranteed after the quantization operation in the same setting.

The other two algorithms used for benchmarking are Q-Push-Gossip, an average consensus scheme, and Q-De-DGD, an optimization algorithm; they are obtained by quantizing the push-sum gossip algorithm and the decentralized subgradient-push algorithm, respectively \cite{taheriquantized}. In the following, we describe Q-De-DGD; Q-Push-Gossip follows the same procedure as Q-De-DGD except it does not require computation and use of a gradient term. 
For consistency, Q-De-DGD here relies on full instead of stochastic gradient. The algorithm is summarized as follows:
\begin{align*}
&Q_i(t) = Q(\x_i(t)-\hat{\x}_i(t)),\qquad
\hat{\x}_i(t+1)  = \hat{\x}_i(t) + Q_i(t) \\
&\mathbf{w}_i(t+1)  = \x_i(t) - \hat{\x}_i(t+1) + [A(t)\x(t)]_i, \qquad
%	x_i(t+1) &= x_i(t) - \hat{x}_i(t+1) + [A(t)y(t)]_i \\
y_i(t+1) = [A(t)y(t)]_i \\
&\z_i(t+1) = \frac{\mathbf{w}_i(t+1)}{y_i(t+1)}, \qquad
\x_i(t+1)  = \mathbf{w}_i(t+1) - \alpha_{t+1} \nabla F_i(\z_i).
\end{align*}
To ensure convergence in a fixed directed network, $\x_i$ and $\hat{\x}_i$ should be initialized as zero vectors, and $y_i$ should be set to $1$ for all $i \in [n]$. However, this scheme is not guaranteed to converge when deployed over time-varying directed networks; indeed, as the results demonstrate, in such setting this scheme does not converge. 
	
Finally, to ensure that the communication costs of quantized algorithms match those of sparsification schemes, we compute the number of communicated bits after quantization in the following way: suppose $s$ is the quantization level for the unbiased stochastic quantization method assigning $\xi_{i}(\x, s)$ to the $i$-th entry, $x_i$, of $\x$ as follows:
\begin{equation*}
	    \xi_{i}(\x, s) = \begin{cases}
	    (\ell+1)/s & \mathrm{w.p. \ } \frac{|x_i|}{\|\x \|_2}s-\ell \\
	    \ell/s & \mbox{otherwise}.
	    \end{cases}
\end{equation*}
Here $0 \leq \ell < s$ and $\frac{|x_i|}{\|\x \|_2}\in [\ell/s, (\ell+1)/s] $. We use $\log(s)+1$ bits for each entry of the vector with one bit allocated for the sign. To match the number of communicated bits of Algorithm \ref{alg:B}, in each quantization protocol we require $64qd = (\log(s)+1)d+32,$
% 	\begin{equation*}
% 	    64qd = (\log(s)+1)d+32,
% \end{equation*}
where $q$ denotes the fraction of entries communicated by the sparsification schemes.
